# Supplementary material for: Worst-Case Complexity of an SQP Method for Nonlinear Equality Constrained Stochastic Optimization
Source: arXiv:2112.14799 source file (2022-01-06)
Supplement: Supplementary file 5 [file appendix.tex]

\section{Proof of Theorem~\ref{th.deterministic} (Deterministic Complexity)}\label{app.deterministic}

In this appendix, we prove Theorem~\ref{th.deterministic}, which states a worst-case complexity bound for Algorithm 2.1 of \cite{ABerahas_FECurtis_DPRobinson_BZhou_2021}.  We refer to quantities defined and employed in the analysis in \cite{ABerahas_FECurtis_DPRobinson_BZhou_2021}.  In particular, in this appendix, $g_k = \nabla f(x_k)$ and $d_k$ is the search direction corresponding to $g_k = \nabla f(x_k)$. Our first lemma gives a lower bound on the change in the model

\begin{lemma}\label{lem:suffdecrease}
  Referring to $\{\kappa_{uv},\kappa_H,\kappa_v,\tau_{\min},\zeta\} \subset (0,\infty)$ and $\sigma \in (0,1)$ from \cite{ABerahas_FECurtis_DPRobinson_BZhou_2021}, let
  \begin{equation} \label{eq:kappahat}
    \hat{\kappa} := \min\left\{1,\frac{1}{(1+\kappa_{uv})\kappa_v\kappa_H^2}\right\}\ \ \text{and}\ \ \kappadec := \min\left\{\sigma \hat{\kappa},
    \tfrac14 \tau_{\min} \zeta \kappa_{uv} \kappa_v \hat{\kappa} \right\}.
  \end{equation}
  For any $\varepsilon \in (0,1)$, if $\|g_k + J_k^\top y_k\| > \varepsilon$ and/or $\sqrt{\|c_k\|_1} > \varepsilon$, then
  \begin{equation} \label{eq:suffdecrease}
    \Delta q(x_k, \tau_k, g_k, H_k, d_k) \geq \kappadec \varepsilon^2.
  \end{equation}
\end{lemma}
\begin{proof}
  Consider arbitrary $(\varepsilon,k) \in (0,1) \times \N{}$ such that $\|g_k + J_k^\top y_k\| > \varepsilon$ and/or $\sqrt{\|c_k\|_1} > \varepsilon$.  Let us consider two cases.  First, suppose that $\|c_k\|_1 > \hat{\kappa} \varepsilon^2$. Then, by \cite[equation (2.9)]{ABerahas_FECurtis_DPRobinson_BZhou_2021},
  \bequationNN
    \Delta q(x_k, \tau_k, g_k, H_k, d_k) \geq \tfrac12 \tau_k \max\{d_k^\top H_k d_k 0\} + \sigma \|c_k\|_1 \geq \sigma \|c_k\|_1 \geq \sigma \hat{\kappa} \varepsilon^2,
  \eequationNN
  which implies \eqref{eq:suffdecrease}, as desired.  Second, suppose that $\|c_k\|_1 \leq \hat{\kappa} \varepsilon^2 \leq \varepsilon^2$, which by the definition of $(\varepsilon,k)$ implies that $\|g_k + J_k^\top y_k\| > \varepsilon$.  It follows from this fact that $\|d_k\| > \varepsilon/\kappa_H$; indeed, if $\|d_k\| \leq \varepsilon/\kappa_H$, then by  \cite[equation (2.6) and Assumption~2.4]{ABerahas_FECurtis_DPRobinson_BZhou_2021} one would find
  \bequationNN
    \|g_k + J_k^\top y_k\| = \|H_k d_k\| \leq \kappa_H \|d_k\| \leq \varepsilon,
  \eequationNN
  which is a contradiction.  Hence, $\|d_k\| > \varepsilon/\kappa_H$, and by \cite[Lemma~2.9]{ABerahas_FECurtis_DPRobinson_BZhou_2021}, it follows that $\|v_k\|^2 \leq \kappa_v \|c_k\| \leq \kappa_v \|c_k\|_1 \leq \kappa_v \hat{\kappa} \varepsilon^2$, which combined shows that
  \bequationNN
    \varepsilon^2/\kappa_H^2 < \|d_k\|^2 = \|u_k\|^2 + \|v_k\|^2 \leq \|u_k\|^2 + \kappa_v \hat{\kappa} \varepsilon^2.
  \eequationNN
  From this fact and the definition of $\hat{\kappa}$, it follows that
  \bequationNN
    \|u_k\|^2 > \frac{\varepsilon^2}{\kappa_H^2} - \kappa_v \hat{\kappa} \varepsilon^2 \geq \frac{\varepsilon^2}{\kappa_H^2}\(1 - \frac{1}{(1+\kappa_{uv})}\) \geq \frac{\kappa_{uv}\varepsilon^2}{(1+\kappa_{uv})\kappa_H^2} \geq \kappa_{uv} \kappa_v \hat{\kappa} \varepsilon^2 \geq \kappa_{uv} \|v_k\|^2,
  \eequationNN
  which along with \cite[Lemma~2.10]{ABerahas_FECurtis_DPRobinson_BZhou_2021} implies $d_k^\top H_k d_k \geq \thalf \zeta \|u_k\|^2 \geq \thalf \zeta \kappa_{uv} \kappa_v \hat{\kappa} \varepsilon^2$.  Thus,
  \begin{align*}
    \Delta q(x_k, \tau_k, g_k, H_k, d_k) &\geq \thalf \tau_k \max\{d_k^\top H_k d_k 0\} + \sigma \|c_k\|_1 \geq \tfrac14 \tau_{\min} \zeta \kappa_{uv} \kappa_v \hat{\kappa} \varepsilon^2,
  \end{align*}
  which implies \eqref{eq:suffdecrease}, as desired. \qed
\end{proof}

We now prove Theorem~\ref{th.deterministic}, further details of which are provided in the statement below.

\begin{theorem}\label{th.deter_complex}
  Theorem~\ref{th.deterministic} holds with \eqref{eq.deterministic_complexity} replaced by
  \bequationNN
    \overline{K}_\varepsilon := \(\frac{\tau_{-1}(f_0 - \flow) + \|c_0\|_1}{\eta \alpha_{\min} \kappadec}\) \varepsilon^{-2} = \(\frac{\tau_{-1}(f_0 - \flow) + \|c_0\|_1}{\min\left\{\eta \alpha_{\min}\sigma \hat{\kappa}, \tau_{\min}(
    \frac14 \eta \alpha_{\min} \zeta \kappa_{uv} \kappa_v \hat{\kappa}) \right\}}\) \varepsilon^{-2},
  \eequationNN
  where $\hat\kappa \in (0,1]$ and $\kappadec \in (0,1)$ are defined in \eqref{eq:kappahat}.
\end{theorem}
\begin{proof}
  To derive a contradiction, suppose \eqref{eq:eps1lon}
does not hold for all $k \in \{0,\dots,\overline{K}_\varepsilon\}$.  Then, along with Lemma~\ref{lem:suffdecrease} and~\cite[equation~(2.10) and Lemma~2.17]{ABerahas_FECurtis_DPRobinson_BZhou_2021}, it follows for all such $k$ that
  \begin{align*}
    \phi (x_k + \alpha_k d_k, \tau_k) &\leq \phi (x_k, \tau_k) - \eta \alpha_k \Delta q(x_k, \tau_k, g_k, H_k, d_k) \\
    &\leq \phi(x_k, \tau_k) - \eta \alpha_{\min} \kappadec \varepsilon^2.
  \end{align*}
  By the definition of $\phi$, this means for all such $k$ that
  \bequationNN
    \tau_k f_{k+1} + \|c_{k+1}\|_1 \leq \tau_k f_k + \|c_k\|_1 - \eta \alpha_{\min} \kappadec \varepsilon^2.
  \eequationNN
  Summing this inequality for all $k \in \{0,\dots,\overline{K}_\varepsilon\}$, one can deduce that
  \bequationNN
    \|c_{\overline{K}_\varepsilon+1}\|_1 - \|c_0\|_1 + \tau_{\overline{K}_\varepsilon}f_{\overline{K}_\varepsilon+1} - \tau_0 f_0 + \sum_{k=1}^{\overline{K}_\varepsilon} f_k (\tau_{k-1} - \tau_k) \leq - (\overline{K}_\varepsilon+1) \eta \alpha_{\min} \kappadec \varepsilon^2.
  \eequationNN
  Since $\{\tau_k\}$ is monotonically nonincreasing, $\|c_{\overline{K}_\varepsilon+1}\|_1 \geq 0$, and $f_k \geq \flow$ for all $k \in \N{}$, it follows from above that
  \bequationNN
    - \|c_0\|_1 + \tau_{\overline{K}_\varepsilon}\flow - \tau_0 f_0 + \flow (\tau_{0} - \tau_{\overline{K}_\varepsilon}) \leq - (\overline{K}_\varepsilon+1) \eta \alpha_{\min} \kappadec \varepsilon^2.
  \eequationNN
  Rearranging this inequality, one arrives at the conclusion that
  \bequationNN
    \overline{K}_\varepsilon+1 \leq \(\frac{\tau_0 (f_0 - \flow) + \|c_0\|_1}{\eta \alpha_{\min} \kappadec}\) \varepsilon^{-2} \leq \(\frac{\tau_{-1} (f_0 - \flow) + \|c_0\|_1}{\eta \alpha_{\min} \kappadec}\) \varepsilon^{-2} \equiv \overline{K}_\varepsilon,
  \eequationNN
  which is a contradiction.  Therefore, one arrives at the desired conclusion that Algorithm 2.1 yields an iterate satisfying \eqref{eq:eps1lon} in at most $\overline{K}_\varepsilon$ iterations. \qed
\end{proof}

%*********
% Section
%*********
\section{Proofs of Lemma \ref{lem:Eksumlsmax} and \ref{lem:Ktaulsmax}} \label{app:probbounds}

In this appendix, we provide proofs of Lemma \ref{lem:Eksumlsmax} and \ref{lem:Ktaulsmax}. In the process of proving these results, we first prove that, for any $\delta \in (0,1)$ and $\hat{\delta}$ as defined (based on $\delta$) in \eqref{eq:hatdelta},
\bequation \label{eq:sumptaudecbound}
    \Prob\left[\sum_{i=0}^{\kmax} \Prob[\Tcal_i < \Tcal_{i-1} | E, G_0,\dots,G_{i-1}] \leq \ell(s_{\max},\hat{\delta})+1 \Bigg| E \right] \geq 1-\delta,
\eequation
where $\ell(\smax,\hat{\delta})$ is defined in \eqref{eq:lsd}.

\iffalse
%Our proof revolves around the construction of a tree where each node at level $k \in \N{}$ is characterized by the history of decreases and history of probabilities of decreases of the merit parameter through iteration $k$ of the algorithm.  
Our goal is to show that an event, denoted as $\Ebad$, occurs with low probability; in particular, for some $\hat{\delta} \in (0,1)$ and with $\smax$ defined as in Assumption \ref{assum:eventE}, we define $\Ebad$ as the event that
\begin{multline}\label{eq:Ebad}
  \left(\sum_{i=0}^{k} \Prob[\Tcal_i < \Tcal_{i-1} | E, G_0,\dots, G_{i-1}] > \ell(s_{\max},\hat{\delta}) + 1\right) \\
  \text{for some}\ \ k \in \{0,\dots,\kmax\}.  
\end{multline}
%\begin{multline}\label{eq:Ebad}
%  \left(\sum_{i=0}^{k} \Prob[\Tcal_i < \Tcal_{i-1} | E, G_0,\dots, G_{i-1}] \geq \ell(s_{\max},\hat{\delta})\right) \land (S_k < s_{\max}) \\
%  \text{for some}\ \ k \in \{0,\dots,\kmax-1\}.  
%\end{multline}
%Note that we do not include $k=k_{\max}$ in this definition of $\Ebad$.

The bulk of our proof focuses on proving that $\Prob[\Ebad | E] \leq \delta$ for some $\delta \in (0,1)$ since, as a consequence of that fact, we have the following result.\footnote{MON: This Lemma seems irrelevant now, maybe just remove it?}

\blemma \label{lem:Ebadsum}
  Let Assumption \ref{assum:eventE} hold and assume $\Prob[\Ebad | E] \leq \delta$ for some $\delta \in (0,1)$. Then,
  \bequation\label{Pgeq}
    \Prob\left[\sum_{i=0}^{\kmax} \Prob[\Tcal_i < \Tcal_{i-1} | E, G_0,\dots,G_{i-1}] \leq \ell(s_{\max},\hat{\delta})+1 \Bigg| E \right] \geq 1-\delta.
  \eequation
\elemma
\bproof
  The result follows trivially from the definition of $\Ebad$.
  %OLD Proof that used to be commented out.
  Let us define the event in the left side of~\eqref{Pgeq} as 
  $$
  E_{\max} := \sum_{i=0}^{\kmax} \Prob[\Tcal_i < \Tcal_{i-1} | E, G_0,\dots,G_{i-1}] 
  \leq \ell(s_{\max},\hat{\delta})+1.
  $$
  To prove the result, our aim is to show that
  \begin{align}\label{eq:PEmax}
    &\Prob\left[E_{\max} \big| E\right] 
    \geq \Prob\left[E_{\max} \land \Ebad^c \big| E\right] 
    = \Prob[\Ebad^c | E] = 1-\Prob[\Ebad | E] \geq 1-\delta.
  \end{align}
  In fact, the first inequality, the second equation, and the final inequality follow from basic probability and the assumptions of the lemma.  All that remains is to prove the first equation.
  
  To prove the first equation,  consider the following mutually exclusive events that exhaustively cover the event $\Ebad^c$:
  \begin{enumerate}
    \item[$E_1$:] $\sum_{i=0}^{k} \Prob[\Tcal_i < \Tcal_{i-1} | E, G_0,\dots, G_{i-1}] < \ell(s_{\max},\hat{\delta})$ for all $k \in \{0,\dots,\kmax-1\}$
    \item[$E_2$:] $S_k = \smax$ for any $k \in \{0,\dots,\kmax-1\}$ such that $\sum_{i=0}^{k} \Prob[\Tcal_i < \Tcal_{i-1} | E, G_0,\dots, G_{i-1}] \geq \ell(s_{\max},\hat{\delta})$
  \end{enumerate}
  We now show that each of these events are subsets of $E_{\max}$.   
  For $E_1$, observe that since $\sum_{i=0}^{k} \Prob[\Tcal_i < \Tcal_{i-1} | E, G_0,\dots, G_{i-1}] < \ell(s_{\max},\hat{\delta})$ for all $k \in \{0,\dots,\kmax-1\}$ and $\Prob[\Tcal_{\kmax} < \Tcal_{\kmax-1} | E, G_0,\dots, G_{\kmax-1}] \leq 1$, it follows that  $\sum_{i=0}^{\kmax} \Prob[\Tcal_i < \Tcal_{i-1} | E, G_0,\dots, G_{i-1}] < \ell(s_{\max},\hat{\delta})+1$, which shows that $E_1 \subseteq E_{\max}$. Next consider any realization in $E_2$.  For that realization, there exists a \emph{smallest} $\kbar \in \{0,\dots,\kmax-1\}$ such that $\sum_{i=0}^{\kbar} \Prob[\Tcal_i < \tau_{i-1} | E, g_0,\dots, g_{i-1}] \geq \ell(s_{\max},\hat{\delta})$ (this follows since the realization is not in $E_1$), and then observe from the definition of $E_2$ that $s_{\kbar} = \smax$.  Note that the definition of $\kbar$ and $\Prob[\Tcal_{\kbar} < \tau_{\kbar-1} | E, g_0,\dots, g_{\kbar-1}] \leq 1$ shows that $\sum_{i=0}^{\kbar} \Prob[\Tcal_i < \tau_{i-1} | E, g_0,\dots, g_{i-1}] < \ell(s_{\max},\hat{\delta}) + 1$.  Next, observe that by the definition of $s_{\max}$ in Assumption~\ref{assum:eventE},\footnote{FEC: I suppose Assumption \ref{assum:eventE} doesn't really say this directly.  Should we make it say it more explicitly?  It could say that if $\smax$ decreases have occurred, then the probability of another decrease is zero.  It may be looser than what we say anyway. DPR: Valid point, fec.  I am fine either way.} $\Prob[\Tcal_i < \tau_{i-1} | E, g_0,\dots, g_{i-1}] = 0$ for all $i \in \{\kbar+1,\dots,\kmax\}$, which combined with our previous observation yields $\sum_{i=0}^{\kmax} \Prob[\Tcal_i < \tau_{i-1} | E, g_0,\dots, g_{i-1}] < \ell(s_{\max},\hat{\delta}) + 1$, i.e., that the realization is also in $E_{\max}$.  In summary, we have proved that $\Ebad^c \equiv E_1\cup E_2 \subseteq E_{\max}$ so that $E_{\max}\land \Ebad^c = \Ebad^c$, establishing the first equality in~\eqref{eq:PEmax} and completing the proof. \qed
\eproof
\fi

As a preliminary result, we state a particular form of Chernoff's bound in the following lemma, which will prove instrumental in deriving \eqref{eq:sumptaudecbound}.

\blemma\label{lem:chernoff}
  For any $k \in \N{}$, let $\{Y_0,\dots,Y_k\}$ be independent Bernoulli random variables.  Then, for any $s \in \N{}_{>0}$ and $\bar{\delta} \in (0,1)$, it follows that
  \bequation \label{eq:chernoffeq1}
    \mu := \sum_{j=0}^k \P[Y_j = 1] \geq \ell(s,\bar{\delta})\ \ \implies \ \ \P\left[\sum_{j=0}^k Y_j \leq s\right] \leq \bar{\delta},
  \eequation
  where $\ell(s,\bar{\delta})$ is defined in \eqref{eq:lsd}.
\elemma
\bproof
  By the multiplicative form of Chernoff's bound, it follows for $\rho := 1 - s/\mu$ (which is in the interval $(0,1)$ by (\ref{eq:chernoffeq1})) that
  \bequationNN
    \P\left[\sum_{j=0}^{k} Y_j \leq s \right] \leq e^{-\frac{\mu \rho^2}{2}} = e^{-\frac{\mu (1-s/\mu)^2}{2}}.
  \eequationNN
  Hence, to prove the result, all that remains is to show that $e^{-\frac{\mu (1-s/\mu)^2}{2}} \leq \bar{\delta}$, i.e.,
  \bequationNN
    -\frac{\mu(1-s/\mu)^2}{2} \leq \log(\bar{\delta})
  \eequationNN
  Using $\log(\bar{\delta}) = -\log(1/\bar{\delta})$, this inequality is equivalent to
  \bequationNN
    0 \leq \frac{\mu(1-s/\mu)^2}{2} - \log(1/\bar{\delta}) = \frac{(\mu - s)^2}{2\mu} - \log(1/\bar{\delta}),
  \eequationNN
  which holds if and only if $\mu^2 - 2\mu (s+\log(1/\bar{\delta})) + s^2 \geq 0$.  Viewing the left-hand side of this inequality as a convex quadratic function in $\mu$, one finds that the inequality holds as long as $\mu$ is greater than or equal to the positive root of the quadratic, i.e.,
  \bequationNN
    \baligned
      \mu
        &\geq s + \log(1/\bar{\delta}) + \sqrt{(s+\log(1/\bar{\delta}))^2 - s^2} \\
        &= s + \log(1/\bar{\delta}) + \sqrt{\log(1/\bar{\delta})^2 + 2s\log(1/\bar{\delta})}.
    \ealigned
  \eequationNN
  Since this holds under assumption in the lemma, the result is proved. \qed
\eproof

Now, we turn our attention to proving \eqref{eq:sumptaudecbound}. For any realization of our algorithm, we define $w_i$ as the number of times the merit parameter was decreased to obtain $x_i$, and $p_i$ as the probability that the merit parameter would be decreased during iteration $i$; we define the \emph{signature} of that realization as $(p_0,\dots,p_{\kmax},w_0,\dots,w_{\kmax})$. The signature of a realization at iteration $k$, i.e. $(p_0,\dots,p_k,w_0,\dots,w_k)$ encodes all of the pertinent information regarding the behavior of the merit parameter sequence up to the start of iteration $k$.

One could imagine using these signatures to define a tree whereby each node contains a subset of all realizations of the algorithm. To construct this tree, first consider the root node, which we denote by $\tilde{N}(p_0,w_0)$, where $p_0$ is uniquely defined by the starting conditions of our algorithm and $w_0 = 0$. All realizations of our algorithm follow the same initialization, so $p_0$ and $w_0$ are in the signature of every realization. Now, we could define a node, $\tilde{N}(p_{[k]},w_{[k]})$, at a depth of $k$ (where the root node has a depth of $0$) in the tree as the set of all realizations of our algorithm for which the signature of the realization at iteration $k$ is exactly $(p_0,\dots,p_k,w_0,\dots,w_k)$. We could then define the edges in our tree by connecting nodes at adjacent levels in the following manner. The node $\tilde{N}(p_{[k]},w_{[k]})$ would be connected to a node a $\tilde{N}(\bar{p}_{[k+1]},\bar{w}_{[k+1]})$ if and only if $p_j = \bar{p}_j$ and $w_j = \bar{w}_j$ for all $j \in \{0,1,\dots,k\}$.

Unfortunately, the construction described in the prior paragraph may lead to all of the nodes in the tree (with the exception of the root node) being sets of zero measure. In order to remedy this, we instead construct a tree where the nodes contain all realizations whose probability signatures fall within specified intervals, rather than the set of realizations that matching these probabilities exactly. To define the intervals, we choose some $B \in \N{}_{>0}$ and restrict the sequence of probabilities $p_{[k]}$ used to define our nodes to:
\begin{equation}
    p_{[k]} = (p_0, \dots, p_k) \in \left\{0, \frac{1}{B}, \dots, \frac{B-1}{B}\right\}^k.
\end{equation}
For a probability $p \in \{0, 1/B, \dots, (B-1)/B\}$, these define the open probability intervals $\iota(p)$:
\begin{equation*}
    \iota(p) = \begin{cases}
        \left[p, p + \frac{1}{B}\right) & \text{if} \;p \in \left\{0, \frac{1}{B}, \dots, \frac{B-2}{B}\right\}, \\
        \left[\frac{B-1}{B}, 1\right] & \text{if} \;p = \frac{B-1}{B}.
    \end{cases}
\end{equation*}

Now, we can construct our tree as follows. As before, first consider the root node, which we denote by $N(p_0,w_0)$, where $p_0 \in \{0, 1/B, \dots, (B-1)/B\}$ is uniquely defined by the starting conditions of our algorithm so that $\Prob[\Tcal_0 < \tau_{-1} | E] \in \iota(p_0)$ and $w_0 = 0$. All realizations of our algorithm follow the same initialization, so there exists $\bar{p}_0 = \Prob[\Tcal_0 < \tau_{-1} | E]$, such that $\bar{p}_0 \in \iota(p_0)$ and $\bar{p}_0$ and $w_0$ are in the signature of every realization. Due to this, we say that the event $x_0 \in N(p_0,w_0)$ occurs with probability one. Now, we can define a node $N(p_{[k]},w_{[k]})$ at a depth of $k$ (where the root node has a depth of 0) in the tree as the set of all realizations of our algorithm for which the signature of the realization at iteration $k$, exactly matches $w_{[k]}$ and falls within the correct probability interval with respect to $p_{[k]}$. More specifically, a realization with signature $(\hat{p}_0,\dots,\hat{p}_k,\hat{w}_0,\dots,\hat{w}_k)$ is a member of $N(p_{[k]},w_{[k]})$ if and only if, for all $j \in [k]$,
\bequationNN
    \hat{p}_j \in \iota(p_j) \quad \text{and} \quad \hat{w}_j = w_j.
\eequationNN
We define the edges in our tree by connecting nodes at adjacent levels in the following manner. The node $N(p_{[k]},w_{[k]})$ is connected to a node a $N(\bar{p}_{[k+1]},\bar{w}_{[k+1]})$ if and only if $p_j = \bar{p}_j$ and $w_j = \bar{w}_j$ for all $j \in [k]$.

Based on the description above, the nodes of our tree satisfy the following definition. For any node at a depth of $k \geq 2$, we say that the event $G_{[k-1]} \in N(p_{[k]},w_{[k]})$ occurs if
\begin{align*}
    &\Prob[\Tcal_k < \Tcal_{k-1} | E, G_{[k-1]}] \in \iota(p_k), \\
    &S_{k-1} = \sum_{i=0}^{k-1} \Ical[\Tcal_i < \Tcal_{i-1}] = w_k, \\
    \text{and}\ \ &G_{[k-2]} \in N(p_{[k-1]},w_{[k-1]}) \text{ occurs as well.}
\end{align*}
In addition, for any node at a depth of $k = 1$, we say that the event $G_{[k-1]} \in N(p_{[k]},w_{[k]})$ occurs if
\begin{align*}
    &\Prob[\Tcal_k < \Tcal_{k-1} | E, G_{[k-1]}] \in \iota(p_k), \\
    &S_{k-1} = \sum_{i=0}^{k-1} \Ical[\Tcal_i < \Tcal_{i-1}] = w_k, \\
    \text{and}\ \ &x_0 \in N(p_{0},w_{0}) \text{ occurs as well.}
\end{align*}
We recall that the only node at a depth of $k=0$ is the root node, which is defined as $N(p_0,w_0)$. By definition, the event $x_0 \in N(p_{0},w_{0})$ occurs with probability one.

\iffalse
Therefore, the signature of any realization of our algorithm is a unique element of the set of all possible signatures
\begin{align*}
\Scal := 
\{(p_0,\dots,p_{\kmax+1}, 
   w_0,\dots,w_{\kmax+1}):  
   p_i \in\{0,1/N,2/N,\dots,1\} \ \text{and} \  
   w_i \in\{0,1,\dots,i\} \}
\end{align*}
which has cardinality $|\Scal| = N^{\kmax+1} (\kmax+1)(\kmax+2)/2$.  We can now define, for each $i \in\{0,1,\dots,\kmax+1\}$, the random vector 
$Y_i : (G_0,\dots,G_i) \to \{0,1/N,2/N,\dots,1\}^{i+1}\times \{0,1,2,\dots,i\}^{i+1}$ by its probability distribution
\begin{align*}
&\ \Prob(Y_i = (p_0,\dots,p_i,w_0,\dots,w_i)) \\
&= \{
\text{fraction of realizations of $(G_0,\dots,G_i)$ with truncated signature $(p_0,\dots,p_i,w_0,\dots,w_i)$}\}.
\end{align*}
In particular, if $\pbar_0$ denotes the fraction of realizations of $G_0$ that cause the merit parameter to decrease during iteration $0$, i.e., $\pbar_0 := \Prob(\Tcal_0 < \tau_{-1})$, then it follows that
\bequationNN
\Prob\big(Y_0 = (\pbar_0,0)\big) = 1
\eequationNN
since with certainty no merit parameter decreases occured to obtain $x_0$ (i.e., $w_ 0 = 0$ for all realizations of the algorithm). We can also notice that 
\begin{align*}
&\Prob(Y_i = (p_0,\dots,p_i,w_0,\dots,w_i)) \\
&= \Prob(Y_{i-1} =  (p_0,\dots,p_{i-1},w_0,\dots,w_{i-1})) \\
&\qquad \cdot
\Prob( 
\Prob( ( \Tcal_i < \tau_{i-1}) = p_k)
\land (S_i = w_i)
\big| Y_{i-1} = (p_0,\dots,p_{i-1},w_0,\dots,w_{i-1})).
\end{align*}
DPR is stopping here because he is not sure if this is any better of a way of going about things.  

\hrule



We now wish to define a tree based on the set of signatures whereby each node will contain a subset of all realizations of the algorithm. Let us now define this tree by describing the nodes and edges.
%\begin{itemize}
    %\item \textbf{Nodes.} 
Level $k$ (starting with $k=0$) of the tree has $N^k k(k+1)/2$ nodes denoted by
    $$
    \{\Ncal(p_0,\dots,p_k,w_0,\dots,w_k): p_i\in\{1/N,2/N,\dots,1\} \ \text{and} \  
   w_i \in\{0,1,\dots,i\}\}.
    $$
    We say that a given realization with signature $(\pbar_0,\dots,\pbar_{\kmax+1},\wbar_0,\dots,\wbar_{\kmax+1})$ is contained in node $\Ncal(p_0,\dots,p_k,w_0,\dots,w_k)$ if $\pbar_i = p_i$ and $\wbar_i = w_i$ for all $i\in\{0,\dots,k\}$. From this definition it follows that if a realization is in node $\Ncal(p_0,\dots,p_k,w_0,\dots,w_k)$ then that realization must also be in node $\Ncal(p_0,\dots,p_j,w_0,\dots,w_j)$ for all $j\leq \{0,\dots,k\}$.  Moreover, the set of \emph{all} realizations is a subset of a \emph{single} node at level zero. For example, let $N = 5$ and suppose that the probability that the merit parameter decreases during iteration $0$ is $2/5$.  Then, it follows that every realization is contained in $\Ncal(2/5,0)$, i.e., no realizations are contained in $\Ncal(1/5,0)$, $\Ncal(3/5,0)$, $\Ncal(4/5,0)$, and $\Ncal(1,0)$.

%    \item \textbf{Edges.} 
Edges are only drawn between nodes at adjacent levels. %In particular, n
Node $\Ncal(p_0,\dots,p_k,w_0,\dots,w_k)$ at level $k$ for $k\in\{0,1,\dots,\kmax\}$ is connected to node $\Ncal(\pbar_0,\dots,\pbar_{k+1},\wbar_0,\dots,\wbar_{k+1})$ at level $k+1$ if and only if $p_j = \pbar_j$ and $w_j = \wbar_j$ for all $j\in\{0,1,\dots,k\}$.
%\end{itemize}

\smallskip
\hrule
\fi

Let us now define certain important sets of nodes in the tree.  First, let
\bequationNN
  \Lgood := \{N(p_{[k]},w_{[k]}) : \left(\sum_{i=0}^k p_i \leq \ell(\smax,\hat{\delta}) + 1\right) \land (w_{k} = s_{\max} \lor k = \kmax)\}
\eequationNN
be the set of nodes at which the sum of the elements of $p_{[k]}$ is sufficiently small and $w_k$ has reached $\smax$ or $k$ has reached $\kmax$.  Second, let
\bequationNN
  \Lbad := \left\{N(p_{[k]},w_{[k]}) : \sum_{i=0}^{k} p_i > \ell(s_{\max},\hat{\delta})+1 \right\}
\eequationNN
be the nodes in the complement of $\Lgood$ at which the sum of the elements of $p_{[k]}$ has exceeded the threshold $\ell(s_{\max},\hat\delta)+1$.


Going forward, we restrict attention to the tree defined by the root node and all paths from the root node that terminate at an element of $\Lgood \cup \Lbad$.  It is clear from this restriction and the definitions of $\Lgood$ and $\Lbad$ that this tree is finite with the elements of $\Lgood \cup \Lbad$ being leaves.

Let us now define relationships between nodes.  The parent of a node is defined as\footnote{dpr:I do not understand this. \textcolor{red}{MON: Hopefully it's fine now?}}
\bequationNN
  P(N(p_{[k]},w_{[k]})) = N(p_{[k-1]},w_{[k-1]}).
\eequationNN
On the other hand, the children of node $N(p_{[k]},w_{[k]})$ are defined as
\begin{multline}
  C(N(p_{[k]},w_{[k]})) = \{N(\hat{p}_{[k+1]}, \hat{w}_{[k+1]}) : \hat{p}_{[k]} = p_{[k]} \text{ and } \hat{w}_{[k]} = w_{[k]}\} \\
  \text{if}\ \ N(p_{[k]},w_{[k]}) \not\in \Lgood \cup \Lbad,
\end{multline}
and $C(N(p_{[k]},w_{[k]})) = \emptyset$ otherwise.  This ensures that paths down the tree indeed terminate at nodes in $\Lgood \cup \Lbad$, making the elements of this union the leaves of the tree.  For convenience in the remainder of our discussions, let $C(\emptyset) = \emptyset$.

We define the height of node $N(p_{[k]},w_{[k]})$ as the length of the longest path from $N(p_{[k]},w_{[k]})$ to a leaf node, i.e., the height is denoted as
\bequationNN
  h(N(p_{[k]},w_{[k]})) := \left(\min \{j \in \N{} \setminus \{0\} : C^j(N(p_{[k]},w_{[k]})) = \emptyset\}\right)-1,
\eequationNN
where $C^j(N(p_{[k]},w_{[k]}))$ is shorthand for applying the mapping $C(\cdot)$ consecutively $j$ times. From this definition, $h(N(p_{[k]},w_{[k]})) = 0$ for all $N(p_{[k]},w_{[k]}) \in \Lgood \cup \Lbad$.

Next, let us define two more sets of nodes that will be useful later; namely, let $C_{dec}(N(p_{[k]},w_{[k]}))$ denote the set of children of $N(p_{[k]},w_{[k]})$ such that $\tau_k < \tau_{k-1}$ and let $\Cdec^c(N(p_{[k]},w_{[k]}))$ denote set of children of $N(p_{[k]},w_{[k]})$ such that $\tau_k = \tau_{k-1}$, so
\begin{align}
  \Cdec(N(p_{[k]},w_{[k]})) := \{
  & N([p_{[k]},p_{k+1}],[w_{[k]},w_{k+1}]) : \nonumber \\
  & (N([p_{[k]},p_{k+1}],[w_{[k]},w_{k+1}]) \in C(N(p_{[k]},w_{[k]}))) \nonumber \\
  & \land (w_{k+1} = w_{k} + 1)\} \label{eq:Cdec}
\end{align}
and
\begin{align}
  \Cdec^c(N(p_{[k]},w_{[k]})) := \{
  & N([p_{[k]},p_{k+1}],[w_{[k]},w_{k+1}]) : \nonumber \\
  & (N([p_{[k]},p_{k+1}],[w_{[k]},w_{k+1}]) \in C(N(p_{[k]},w_{[k]}))) \nonumber \\
  & \land (w_{k+1} = w_{k})\}. \label{eq:CdecC}
\end{align}

Finally, for any $\hat{\delta} \in (0,1)$, we define the event, $\EbadB$, as the event that
\begin{multline}\label{eq:EbadB}
  \left(\sum_{i=0}^{k} \Prob[\Tcal_i < \Tcal_{i-1} | E, G_{[i-1]}] > \ell(s_{\max},\hat{\delta}) +  \frac{\kmax+1}{B} + 1\right) \\
  \text{for some}\ \ k \in [\kmax].  
\end{multline}
We will prove that, for any $B \in \N{}_{>0}$, $\Prob[\EbadB] \leq \delta$ holds when $\hat{\delta}$ is computed by \eqref{eq:hatdelta}.

Let us now prove some properties of the leaf nodes.

\blemma \label{lem:leafnodes}
  Let Assumption \ref{assum:eventE} hold. Then,
  \bequationNN
    \Prob[G_{[k-1]} \in N(p_{[k]},w_{[k]}) \land \EbadB | E] = 0\ \ \text{for all}\ \ N(p_{[k]},w_{[k]}) \in \Lgood
  \eequationNN
  and
  \begin{align*}
    &\Prob[G_{[k-1]} \in N(p_{[k]},w_{[k]}) \land \EbadB | E] \\
    &\leq \hat{\delta} \prod_{i=1}^k \Prob\left[\Prob[\Tcal_i < \Tcal_{i-1} | E, G_{[i-1]}] \in \iota(p_i) \big| E, S_{i-1} = w_{i}, G_{[i-2]} \in N(p_{[i-1]},w_{[i-1]})\right] \\
    & \text{for all}\ \ N(p_{[k]},w_{[k]}) \in \Lbad.
  \end{align*}
\elemma
\bproof
  Consider arbitrary $k \in \N{}$ and $(p_{[k]},w_{[k]})$ with $N(p_{[k]},w_{[k]}) \in \Lgood$.  By the definition of $\Lgood$, it follows that,
  \begin{equation*}
    \sum_{i=0}^k p_i \leq \ell(\smax, \hat{\delta}) + 1.
  \end{equation*}
  Therefore, since the maximum depth of a node is $\kmax$,
  \begin{align*}
    &\Prob\left[\sum_{i=0}^k \Prob[\Tcal_i < \Tcal_{i-1} | E, G_{[i-1]}] > \ell(\smax,\hat{\delta}) + \frac{\kmax+1}{B} + 1 \Big| E, G_{[k-1]} \in N(p_{[k]},w_{[k]})\right] \\
    &\leq \Prob\left[\sum_{i=0}^k \left(p_i + \frac{1}{B}\right) > \ell(\smax,\hat{\delta}) + \frac{\kmax+1}{B} + 1 \Big| E, G_{[k-1]} \in N(p_{[k]},w_{[k]})\right] \\
    &\leq \Prob\left[\ell(\smax,\hat{\delta}) + \frac{k+1}{B} + 1 > \ell(\smax,\hat{\delta}) + \frac{\kmax+1}{B} + 1 \Big| E, G_{[k-1]} \in N(p_{[k]},w_{[k]})\right] \\
    &\leq \Prob\left[\ell(\smax,\hat{\delta}) + \frac{\kmax+1}{B} + 1 > \ell(\smax,\hat{\delta}) + \frac{\kmax+1}{B} + 1 \Big| E, G_{[k-1]} \in N(p_{[k]},w_{[k]})\right] \\
    &= 0.
  \end{align*}
  In addition, for any $j \in \{1,\dots,k\}$, by the definitoin of conditional probability,
  \begin{align*}
    &\Prob\left[G_{[j-1]} \in N(p_{[j]},w_{[j]}) \land \EbadB \;\text{occurs at iteration $j$} | E\right] \\
    &=\Prob\left[\sum_{i=0}^{j} \Prob[\Tcal_i < \Tcal_{i-1} | E, G_{[i-1]}] > \ell(\smax,\hat{\delta}) + \frac{\kmax+1}{B} + 1 \Big| E, G_{[j-1]} \in N(p_{[j]},w_{[j]})\right] \\
    &\quad \cdot \Prob\left[G_{[j-1]} \in N(p_{[j]},w_{[j]}) | E\right] \\
    &= 0.
  \end{align*}
  We also note that $\EbadB$ can never occur at $j=0$ since $\ell(\smax,\hat{\delta})+1 > 1$ and therefore $\EbadB$ does not occur for any $G_{[j-1]}$ with $j \in \{0,\dots,k\}$ in any node on the path leading from the root node to $N(p_{[k]},w_{[k]})$. Moreover, by the defintion of $\Lgood$, at least one of $w_{k} = \smax$ or $k = \kmax$ holds. When $k = \kmax$, it follows by the preceding argument that 
  \begin{equation*}
    \Prob\left[\sum_{i=0}^{\kmax} \Prob[\Tcal_i < \Tcal_{i-1} | E, G_{[i-1]}] \leq \ell(\smax,\hat{\delta}) + \frac{\kmax+1}{B} + 1 \Big| E, G_{[k-1]} \in N(p_{[k]},w_{[k]})\right] = 1,
  \end{equation*}
  holds, so that $\EbadB$ cannot occur in this case. On the other hand, when $w_{k} = \smax$ holds, by Assumption \ref{assum:eventE}, $\Prob[\Tcal_i < \Tcal_{i-1} | E, G_{[i-1]}] = 0$ holds for all $i \geq k$. Therefore,
  \begin{equation*}
    \Prob\left[\sum_{i=0}^{\kmax} \Prob[\Tcal_i < \Tcal_{i-1} | E, G_{[i-1]}] \leq \ell(\smax,\hat{\delta}) + \frac{\kmax+1}{B} + 1 \Big| E, G_{[k-1]} \in N(p_{[k]},w_{[k]})\right] = 1,
  \end{equation*}
  follows in this case as well and $\EbadB$ cannot occur. Overall, it follows that
  \bequationNN
    \Prob[G_{[k-1]} \in N(p_{[k]},w_{[k-1]}) \land \EbadB | E] = 0,
  \eequationNN
  which is the first desired conclusion.
  
  \iffalse
  since $N(p_{[k]},w_{[k]}) \in \Lgood$, it follows that $P(N(p_{[k]},w_{[k-1]})) \not\in \Lbad$ due to the fact that $C(P(N(p_{[k]},w_{[k-1]}))) \neq \emptyset$ whereas the elements of $\Lbad$ are leaf nodes.  Therefore, $\sum_{i=0}^{k-2} p_i \leq \ell(\smax,\hat{\delta})$.  This means that for any $G_{[k-1]} \in N(p_{[k]},w_{[k-1]})$ one finds
  \bequationNN
    \sum_{i=0}^{k-2} \Prob[\Tcal_i < \Tcal_{i-1} | E, G_0,\dots, G_{i-1}] \leq \ell(s_{\max},\hat{\delta}),
  \eequationNN
  from which it follows that $\Ebad$ does not occur for any $G_{[j-1]}$ with $j \in \{0,\dots,k-2\}$ in any node on a path leading from the root node to $N(p_{[k]},w_{[k]})$.  Let us now consider two cases.  First, if $k=\kmax+1$, then it follows from the preceding arguments that $\Ebad$ does not occur for any $G_{[j-1]}$ with $j \in \{0,\dots,\kmax-1\}$ in any node on the path from the root to $N(p_{[k]},w_{[k-1]})$.  Since, by definition, $\Ebad$ only occurs for $k \in \{0,\dots,\kmax-1\}$, this means that $\Ebad$ does not occur in any node on a path from the root to $N(p_{[k]},w_{[k-1]})$.  Second, if $w_{k-1} = \smax$, then it follows by the definition of $\Ebad$ and the preceding arguments that $\Ebad$ does not occur in any node on a path from the root node that includes $N(p_{[k]},w_{[k-1]})$.  Overall, it follows that
  \bequationNN
    \Prob[G_{[k-1]} \in N(p_{[k]},w_{[k-1]}) \land \Ebad | E] = 0,
  \eequationNN
  which is the first desired conclusion.
  \fi

  Now consider arbitrary $k \in \N{}$ and $(p_{[k]},w_{[k]})$ with $N(p_{[k]},w_{[k]}) \in \Lbad$.  By the definition of conditional probability, we have
  \begin{align*}
    &\Prob[G_{[k-1]} \in N(p_{[k]},w_{[k]}) \land \EbadB | E] \\
    &= \Prob[\EbadB | E, G_{[k-1]} \in N(p_{[k]},w_{[k]})] \Prob[G_{[k-1]} \in N(p_{[k]},w_{[k]}) | E] \\
    &\leq \Prob[G_{[k-1]} \in N(p_{[k]},w_{[k]}) | E].
  \end{align*}
  Then, using the initial condition that $x_0 \in N(p_0,w_0)$, it follows that
  \begin{align}
    &\Prob[G_{[k-1]} \in N(p_{[k]},w_{[k]}) \land \EbadB | E] \nonumber \\
    &\leq \Prob[G_{[k-1]} \in N(p_{[k]},w_{[k]}) | E] \nonumber \\
    &= \Prob\left[(\Prob[\Tcal_{k} < \Tcal_{k-1} | E, G_{[k-1]}] \in  \iota(p_k)) \land S_{k-1} = w_{k} \land G_{[k-2]} \in N(p_{[k-1]},w_{[k-1]}) \big| E\right] \nonumber \\
    &= \Prob\left[\Prob[\Tcal_{k} < \Tcal_{k-1} | E, G_{[k-1]}] \in \iota(p_k) \big| E, S_{k-1} = w_{k}, G_{[k-2]} \in N(p_{[k-1]},w_{[k-1]})\right] \nonumber \\
    &\quad \cdot\Prob\left[S_{k-1} = w_{k} \land G_{[k-2]} \in N(p_{[k-1]},w_{[k-1]}) \big| E\right] \nonumber \\
    &= \Prob\left[\Prob[\Tcal_{k} < \Tcal_{k-1} | E, G_{[k-1]}] \in \iota(p_k) \big| E, S_{k-1} = w_{k}, G_{[k-2]} \in N(p_{[k-1]},w_{[k-1]})\right] \nonumber \\
    &\quad \cdot\Prob\left[S_{k-1} = w_{k} \big| E, G_{[k-2]} \in N(p_{[k-1]},w_{[k-1]})\right]
    \Prob\left[G_{[k-2]} \in N(p_{[k-1]},w_{[k-1]}) \big| E\right] \nonumber \\
    &= \Prob[x_0 \in N(p_0,w_0)] \prod_{i=1}^k \Big(\Prob\left[\Prob[\Tcal_{i} < \Tcal_{i-1} | E, G_{[i-1]}] \in \iota(p_i) \big| E, S_{i-1} = w_{i}, G_{[i-2]} \in N(p_{[i-1]},w_{[i-1]})\right] \nonumber \\
    &\qquad \cdot \Prob\left[S_{i-1} = w_{i} \big| E, G_{[i-2]} \in N(p_{[i-1]},w_{[i-1]})\right]\Big) \nonumber \\
    &= \prod_{i=1}^k \Big(\Prob\left[\Prob[\Tcal_{i} < \Tcal_{i-1} | E, G_{[i-1]}] \in \iota(p_i) \big| E, S_{i-1} = w_{i}, G_{[i-2]} \in N(p_{[i-1]},w_{[i-1]})\right] \nonumber \\
    &\qquad \cdot \Prob\left[S_{i-1} = w_{i} \big| E, G_{[i-2]} \in N(p_{[i-1]},w_{[i-1]})\right]\Big). \label{eq:smax1proof1}
  \end{align}
    
  Next, define
  \bequationNN
    \baligned
      \Idec &:= \{i : (i \in \{1,\dots,k\}) \land (w_{i} = w_{i-1} + 1)\} \\ \text{and}\ \ 
    \Idec^c &:= \{i : (i \in \{1,\dots,k\}) \land (w_{i} = w_{i-1})\},
    \ealigned
  \eequationNN
  which by the definition of $w_{[k]}$ form a partition of $\{1,\dots,k\}$. For any $i \in \Idec$,
  \begin{align*}
    &\quad \ \Prob[S_{i-1} = w_{i} | E, G_{[i-2]} \in N(p_{[i-1]},w_{[i-1]})] \\
    &= \Prob[\Tcal_{i-1} < \Tcal_{i-2} |E,  G_{[i-2]} \in N(p_{[i-1]},w_{[i-2]})] \\
    &\leq p_{i-1} + \frac{1}{B}.
  \end{align*}
  On the other hand, for any $i \in \Idec^c$,
  \begin{align*}
    &\ \Prob[S_{i-1} = w_{i} | E, G_{[i-2]} \in N(p_{[i-1]},w_{[i-1]})] \\
    =&\ \Prob[\Tcal_{i-1} = \Tcal_{i-2} |E,  G_{[i-2]} \in N(p_{[i-1]},w_{[i-1]})] \\
    =&\ 1 - \Prob[\Tcal_{i-1} < \Tcal_{i-2} |E,  G_{[i-2]} \in N(p_{[i-1]},w_{[i-1]})] \leq 1-p_{i-1}.
  \end{align*}
  Thus, it follows that
  \bequationNN
    \prod_{i=1}^{k} \Prob[S_{i-1} = w_{i} | E, G_{[i-2]} \in N(p_{[i-1]},w_{[i-1]})] \leq \(\prod_{i \in \Idec} p_{i-1} + \frac{1}{B}\) \(\prod_{j \in \Idec^c} (1-p_{j-1})\).
  \eequationNN
    
  By the definition of $\Lbad$, we have
  \bequationNN
    \sum_{i=0}^k p_i > \ell(\smax,\hat{\delta}) + 1.
  \eequationNN
  Combining this with the fact that $p_k \in [0,1]$ by definition, implies
  \bequationNN
    \sum_{i=0}^{k-1} p_i > \ell(\smax,\hat{\delta}).
  \eequationNN
  In addition, by the definition of $\smax$ in Assumption \ref{assum:eventE}, we have $w_k \leq \smax$, from which it follows that $|\Idec| \leq \smax$.
    
  Now, let $Z_0,\dots,Z_{k-1}$ be independent Bernoulli random variables with
  \begin{equation*}
    \Prob[Z_i=1] = \begin{cases} p_i + \frac{1}{B} & \text{if} \; i+1 \in \Idec \\
    p_i & \text{if} \; i+1 \in \Idec^c
    \end{cases}
  \end{equation*}
  for all $i=0,\dots,k-1$. Clearly, from this definition we have $\sum_{i=0}^{k-1} \Prob[Z_i=1] \geq \ell(\smax, \hat{\delta})$. Then, it follows by Lemma \ref{lem:chernoff} and the preceding argument that
  \begin{align*}
    &\prod_{i \in \Idec} \left(p_{i-1} + \frac{1}{B}\right) \prod_{j \in \Idec^c} (1-p_{j-1}) \\
    &= \Prob\left[(Z_{i-1} = 1 \;\forall i \in \Idec) \land (Z_{j-1} = 0 \; \forall j \in \Idec^c) \right] \\
    &= \Prob\left[\sum_{r=0}^{k-1} Z_r \leq \smax \land (Z_{i-1} = 1 \;\forall i \in \Idec) \land (Z_{j-1} = 0 \; \forall j \in \Idec^c) \right] \\
    &\leq \Prob\left[\sum_{i=0}^{k-1} Z_i \leq \smax\right] \leq \hat{\delta}.
  \end{align*}
    %\bequationNN
    %    \prod_{i \in \Idec} p_{i-1} \prod_{r \in \Idec^c} (1-p_{r-1}) \leq \Prob\left[\sum_{i=0}^{k-1} Z_i < \smax\right] \leq \hat{\delta}. \footnote{If this statement is a bit confusing, you can just think of this as saying that the $\tau$ decreases line up with some realization of the $Z_i$'s such that they do not sum up to $\smax$. Again, for $\smax = 1$, $\Idec = \emptyset$ so that the left hand side is simply $\prod_{i=1}^k 1-p_i$ and the first inequality is an equality.}
    %\eequationNN
  Combining this with \eqref{eq:smax1proof1}, it follows that
  \begin{align*}
    &\Prob[G_{[k-1]} \in N(p_{[k]},w_{[k]}) \land \EbadB | E] \\
    &\leq \hat{\delta} \prod_{i=1}^k \Prob\left[\Prob[\Tcal_i < \Tcal_{i-1} | E, G_{[i-1]}] \in \iota(p_i) \big| E, S_{i-1} = w_{i}, G_{[i-2]} \in N(p_{[i-1]},w_{[i-1]})\right],
  \end{align*}
  which is the second desired conclusion. \qed
\eproof

Next, we present a lemma about nodes in the sets defined in \eqref{eq:Cdec} and \eqref{eq:CdecC}.  The lemma essentially states that a certain probability of interest, defined as the product of probabilities along a path to a child node, can be reduced to a product of probabilities to the child's parent node by partitioning the childen into those at which a merit parameter decrease has occurred and children at which a merit parameter decrease has not occurred.

\blemma \label{lem:cdec}
  Let Assumption \ref{assum:eventE} hold.  Then, given $(p_{[k]},w_{[k]})$, it follows that
  \begin{align*}
    &\sum_{\{(p_{k+1},w_{k+1}) : N(p_{[k+1]},w_{[k+1]}) \in \Cdec(N(p_{[k]},w_{[k]})) \}} \\
    &\prod_{i=1}^{k+1} \Prob\left[\Prob[\Tcal_{i} < \Tcal_{i-1} | E, G_{[i-1]}] \in \iota(p_i) \big| E, S_{i-1} = w_{i}, G_{[i-2]} \in N(p_{[i-1]},w_{[i-1]})\right] \\
    &\quad= \prod_{i=1}^k \Prob\left[\Prob[\Tcal_{i} < \Tcal_{i-1} | E, G_{[i-1]}] \in \iota(p_i) \big| E, S_{i-1} = w_{i}, G_{[i-2]} \in N(p_{[i-1]},w_{[i-1]})\right]
  \end{align*}
  and similarly
  \begin{align*}
    &\sum_{\{(p_{k+1},w_{k+1}) : N(p_{[k+1]},w_{[k+1]}) \in \Cdec^c(N(p_{[k]},w_{[k]})) \}} \\
    &\prod_{i=1}^{k+1} \Prob\left[\Prob[\Tcal_{i} < \Tcal_{i-1} | E, G_{[i-1]}] \in \iota(p_i) \big| E, S_{i-1} = w_{i}, G_{[i-2]} \in N(p_{[i-1]},w_{[i-1]})\right] \\
    &\quad= \prod_{i=1}^k \Prob\left[\Prob[\Tcal_{i} < \Tcal_{i-1} | E, G_{[i-1]}] \in \iota(p_i) \big| E, S_{i-1} = w_{i}, G_{[i-2]} \in N(p_{[i-1]},w_{[i-1]})\right],
  \end{align*}
  where by the definitions of $\Cdec$ and $\Cdec^c$ it follows that the value of $w_{k+1}$ in the sum in the former equation is one greater than the value of $w_{k+1}$ in the sum in the latter equation.
\elemma
\bproof
  We prove the former statement and claim that the latter statement can be proved similarly.  For any $(p_{k+1},w_{k+1})$ such that $N(p_{[k+1]},w_{[k+1]}) \in C(N(p_{[k]},w_{[k]}))$, it follows that
  \begin{align*}
    &\sum_{N(p_{[k+1]},w_{[k+1]}) \in \Cdec(N(p_{[k]},w_{[k]}))} \\
    &\prod_{i=1}^{k+1} \Prob\left[\Prob[\Tcal_{i} < \Tcal_{i-1} | E, G_{[i-1]}] \in \iota(p_i) \big| E, S_{i-1} = w_{i}, G_{[i-2]} \in N(p_{[i-1]},w_{[i-1]})\right] \\
    &= \prod_{i=1}^{k} \Prob\left[\Prob[\Tcal_{i} < \Tcal_{i-1} | E, G_{[i-1]}] \in \iota(p_i) \big| E, S_{i-1} = w_{i}, G_{[i-2]} \in N(p_{[i-1]},w_{[i-1]})\right] \\
    &\qquad \cdot \sum_{N(p_{[k+1]},w_{[k+1]}) \in \Cdec(N(p_{[k]},w_{[k]}))} \\
    &\qquad\qquad \Prob\left[\Prob[\Tcal_{k+1} < \Tcal_{k} | E, G_{[k]}] \in \iota(p_{k+1}) \big| E, S_{k} = w_{k+1}, G_{[k-1]} \in N(p_{[k]},w_{[k]})\right].
  \end{align*}
  The desired conclusion follows since, by the definition of $\Cdec(N(p_{[k]},w_{[k]}))$, all nodes in this set have $S_k = w_{k+1} = w_{k}+1$, meaning that the sum on the right-hand side is the sum of all conditional probabilities with the same conditions, and hence the sum is 1.
  
  The proof for $\Cdec^c$ follows in the same manner with $\Cdec^c$ in place of $\Cdec$ and $S_k=w_{k+1}=w_{k}$ in place of $S_k=w_{k}=w_{k-1}+1$. \qed
\eproof

Next, we derive a result for any node where $w_{k} = \smax - 1$.

\blemma \label{lem:smaxw1}
  Let Assumption \ref{assum:eventE} hold.  For any $(p_{[k]},w_{[k]})$ such that $w_{k} = s_{\max} - 1$ and $N(p_{[k]},w_{[k]}) \not\in \Lgood$, it follows that
  \begin{align}
    &\Prob[G_{[k-1]} \in N(p_{[k]},w_{[k]}) \land \EbadB | E] \nonumber \\
    &\leq \hat{\delta} \prod_{i=1}^k \Prob\left[\Prob[\Tcal_{i} < \Tcal_{i-1} | E, G_{[i-1]}] \in \iota(p_i) \big| E, S_{i-1} = w_{i}, G_{[i-2]} \in N(p_{[i-1]},w_{[i-1]})\right].  \label{eq:recursivebound1}
  \end{align}
\elemma
\bproof
  By Lemma \ref{lem:leafnodes} and the supposition that $N(p_{[k]},w_{[k]}) \not\in \Lgood$, it follows that the result holds for all $(p_{[k]},w_{[k]})$ such that $h(N(p_{[k]},w_{[k]})) = 0$.  With this base case being established, we now prove the result by induction on $h(N(p_{[k]},w_{[k]}))$.  Suppose that the result holds for all $(p_{[k]},w_{[k]})$ such that $w_{k} = s_{\max} - 1$, $N(p_{[k]},w_{[k]}) \not\in \Lgood$, and $h(N(p_{[k]},w_{[k]})) \leq j$ for some $j \in \N{}$.  Our goal is to show that the same statement holds with $j$ replaced by $j+1$.  For this purpose, consider arbitrary $(p_{[k]},w_{[k]})$ such that $w_{k} = s_{\max} - 1$, $N(p_{[k]},w_{[k]}) \not\in \Lgood$, and $h(N(p_{[k]},w_{[k]})) = j + 1$.  Observe that by the definition of the child operators $C$, $\Cdec$, and $\Cdec^c$, it follows that
  \begin{align*}
    &\Prob[G_{[k-1]} \in N(p_{[k]},w_{[k]}) \land \EbadB | E] \\
    &= \sum_{\{(p_{k+1},w_{k+1}) : N(p_{[k+1]},w_{[k+1]}) \in C(N(p_{[k]},w_{[k]})) \}} \Prob[G_{[k]} \in N(p_{[k+1]},w_{[k+1]}) \land \EbadB | E] \\
    &= \sum_{\{(p_{k+1},w_{k+1}) : N(p_{[k+1]},w_{[k+1]}) \in \Cdec(N(p_{[k]},w_{[k]})) \}} \Prob[G_{[k]} \in N(p_{[k+1]},w_{[k+1]}) \land \EbadB | E] \\
    &+ \sum_{\{(p_{k+1},w_{k+1}) : N(p_{[k+1]},w_{[k+1]}) \in \Cdec^c(N(p_{[k]},w_{[k]})) \}} \Prob[G_{[k]} \in N(p_{[k+1]},w_{[k+1]}) \land \EbadB | E].
  \end{align*}
  Since $w_{k} = \smax-1$, it follows from the definition of $\Cdec$ that for any $(p_{k+1},w_{k+1})$ with $N(p_{[k+1]},w_{[k+1]}) \in \Cdec(N(p_{[k]},w_{[k]}))$, one finds that $w_{k+1} = w_{k}+1 = \smax$. By the definition of $\smax$ in Assumption \ref{assum:eventE}, this implies that $\Prob[\Tcal_{k+1} < \Tcal_k | E, G_{[k]}] = 0$ so that $p_{k+1} = 0$. In addition, since $N(p_{[k]},w_{[k]}) \not\in \Lbad$ since $C(N(p_{[k]},w_{[k]})) \neq \emptyset$, it follows that $\sum_{i=0}^{k+1} p_{k+1} \leq \ell(\smax,\hat{\delta})+1$, meaning $N(p_{[k+1]},w_{[k+1]}) \in \Lgood$.  Consequently, from above and Lemma \ref{lem:leafnodes}, one finds
  \begin{align*}
    &\Prob[G_{[k-1]} \in N(p_{[k]},w_{[k]}) \land \EbadB | E] \\
    &= \sum_{\{(p_{k+1},w_{k+1}) : N(p_{[k+1]},w_{[k+1]}) \in \Cdec^c(N(p_{[k]},w_{[k]})) \}} \Prob[G_{[k]} \in N(p_{[k+1]},w_{[k+1]}) \land \EbadB | E].
  \end{align*}
  Since $h(N(p_{[k]},w_{[k]}) = j+1$, it follows that $h(N(p_{[k+1]},w_{[k+1]})) \leq j$ for any $(p_{[k+1]},w_{[k+1]})$ with $h(N(p_{[k+1]},w_{[k+1]})) \in \Cdec^c(N(p_{[k]},w_{[k]}))$.  Therefore, by the induction hypothesis and the result of Lemma~\ref{lem:cdec}, it follows that
  \begin{align*}
    &\Prob[G_{[k-1]} \in N(p_{[k]},w_{[k]}) \land \EbadB | E] \\
    &= \sum_{\{(p_{k+1},w_{k+1}) : N(p_{[k+1]},w_{[k+1]}) \in \Cdec^c(N(p_{[k]},w_{[k]})) \}} \\
    &\quad \hat{\delta} \prod_{i=1}^{k+1} \Prob\left[\Prob[\Tcal_{i} < \Tcal_{i-1} | E, G_{[i-1]}] \in \iota(p_i) \big| E, S_{i-1} = w_{i}, G_{[i-2]} \in N(p_{[i-1]},w_{[i-1]})\right] \\
    &\quad\leq \hat{\delta} \prod_{i=1}^k \Prob\left[\Prob[\Tcal_{i} < \Tcal_{i-1} | E, G_{[i-1]}] \in \iota(p_i) \big| E, S_{i-1} = w_{i}, G_{[i-2]} \in N(p_{[i-1]},w_{[i-1]})\right],
  \end{align*}
  which completes the proof. \qed
\eproof

\iffalse
We can now prove our main result for $\smax = 1$, which serves as the base case for an induction that we use to prove the result for larger $\smax$.

\begin{corollary}
  Let Assumption \ref{assum:eventE} hold and suppose $\smax = 1$. Then,
  \bequationNN
  \Prob[\Ebad | E] \leq \hat{\delta}
  \eequationNN
  and
  \bequationNN
    \Prob\left[\sum_{i=0}^{\kmax} \Prob[\Tcal_i < \Tcal_{i-1} | E, G_0,\dots,G_{i-1}] \leq \ell(s_{\max},\hat{\delta})+1 \Bigg| E \right] \geq 1-\hat{\delta}.
  \eequationNN
\end{corollary}
\bproof
  The first result follows by applying Lemma \ref{lem:smaxw1} for $(p_0,w_0)$ corresponding to the root note $N(p_0,w_0)$.  The second result then follows with Lemma~\ref{lem:Ebadsum}. \qed
\eproof
\fi

Using the preceding lemma as a base case, we now perform induction on the difference $\smax - w_{k}$ to prove a similar result for arbitrary $\smax$.

\blemma \label{lem:nodeprobfull}
  Let Assumption \ref{assum:eventE} hold.  For any $(p_{[k]},w_{[k]})$ such that $N(p_{[k]},w_{[k]}) \not\in \Lgood$, it follows that
  \begin{align*}
    &\Prob[G_{[k-1]} \in N(p_{[k]},w_{[k]}) \land \EbadB | E] \\
    &\leq \hat{\delta} \cdot \sum_{j=0}^{\min\{\smax-w_{k}-1,h(N(p_{[k]},w_{[k]}))\}} \( \begin{matrix} h(N(p_{[k]},w_{[k]})) \\ j \end{matrix} \) \\
    &\qquad \cdot \prod_{i=1}^k \Prob\left[\Prob[\Tcal_{i} < \Tcal_{i-1} | E, G_{[i-1]}] \in \iota(p_i) \big| E, S_{i-1} = w_{i}, G_{[i-2]} \in N(p_{[i-1]},w_{[i-1]})\right].
  \end{align*}
\elemma
\bproof
  For all $(p_{[k]},w_{[k]})$ such that $N(p_{[k]},w_{[k]}) \not\in \Lgood$ and $h(N(p_{[k]},w_{[k]})) = 0$, it follows that $N(p_{[k]},w_{[k]}) \in \Lbad$.  The result holds in this case according to Lemma~\ref{lem:leafnodes} since one finds that $\sum_{j=0}^{\min\{\smax-w_{k}-1,h(N(p_{[k]},w_{[k]}))\}} \binom{h(N(p_{[k]},w_{[k]}))}{j} = \binom{0}{0} = 1$.  On the other hand, for all $(p_{[k]},w_{[k]})$ such that $N(p_{[k]},w_{[k]}) \not\in \Lgood$ and $\smax - w_{k} = 1$, the result follows from Lemma~\ref{lem:smaxw1}.  Hence, to prove the remainder of the result by induction, we need only assume that it holds for all $(p_{[k]},w_{[k]})$ such that $N(p_{[k]},w_{[k]}) \not\in \Lgood$, $h(N(p_{[k]},w_{[k]})) \leq t$ for some $t \in \N{}$, and $\smax - w_{k} = r$ for some $r \in \N{} \setminus \{0\}$ and show that it holds for all $(p_{[k]},w_{[k]})$ such that $N(p_{[k]},w_{[k]}) \not\in \Lgood$, $h(N(p_{[k]},w_{[k]})) = t + 1$, and $\smax - w_{k} = r$.  This is our aim in the remainder of the proof.
  
  Consider arbitrary $(p_{[k]},w_{[k]})$ such that $N(p_{[k]},w_{[k]}) \not\in \Lgood$, $h(N(p_{[k]},w_{[k]})) = t + 1$, and $\smax - w_{k} = r$.  By the definitions of $C$, $\Cdec$, and $\Cdec^c$, it follows that
  \begin{align*}
    &\Prob[G_{[k-1]} \in N(p_{[k]},w_{[k]}) \land \EbadB | E] \\
    &= \sum_{\{(p_{[k+1]},w_{[k+1]}) : N(p_{[k+1]},w_{[k+1]}) \in C(N(p_{[k]},w_{[k]})) \}} \Prob[G_{[k]} \in N(p_{[k+1]},w_{[k+1]}) \land \EbadB | E] \\
    &= \sum_{\{(p_{[k+1]},w_{[k+1]}) : N(p_{[k+1]},w_{[k+1]}) \in \Cdec(N(p_{[k]},w_{[k]})) \}} \Prob[G_{[k]} \in N(p_{[k+1]},w_{[k+1]}) \land \EbadB | E] \\
    &+ \sum_{\{(p_{[k+1]},w_{[k+1]}) : N(p_{[k+1]},w_{[k+1]}) \in \Cdec^c(N(p_{[k]},w_{[k]})) \}} \Prob[G_{[k]} \in N(p_{[k+1]},w_{[k+1]}) \land \EbadB | E].
  \end{align*}
  Further by the definition of $\Cdec$, it follows that $w_{k+1} = w_k + 1$ (thus $\smax - w_{k+1} = r-1$) for all terms in the former sum on the right-hand side, whereas by the definition of $\Cdec^c$ it follows that $w_{k+1} = w_k$ (thus $\smax - w_{k+1} = r$) for all terms in the latter sum on the right-hand side.  Moreover, from $h(N(p_{[k]},w_{[k]})) = t+1$, it follows that $h(N(p_{[k+1]},w_{[k+1]})) \leq t$ for all terms on the right-hand side.  Therefore, by the induction hypothesis, it follows that
  \begin{align*}
    &\Prob[G_{[k-1]} \in N(p_{[k]},w_{[k]}) \land \EbadB | E] \\
    &\leq \sum_{\{(p_{[k+1]},w_{[k+1]}) : N(p_{[k+1]},w_{[k+1]}) \in \Cdec(N(p_{[k]},w_{[k]})) \}} \hat{\delta} \sum_{j=0}^{\min\{r-2,t\}} \binom{t}{j} \\
    &\quad \cdot \prod_{i=1}^{k+1} \Prob\left[\Prob[\Tcal_{i} < \Tcal_{i-1} | E, G_{[i-1]}] \in \iota(p_{i}) \big| E, S_{i-1} = w_i, G_{[i-2]} \in N(p_{[i-1]},w_{[i-1]})\right] \\
    &+ \sum_{\{(p_{[k+1]},w_{[k+1]}) : N(p_{[k+1]},w_{[k+1]}) \in \Cdec^c(N(p_{[k]},w_{[k]})) \}} \hat{\delta} \sum_{j=0}^{\min\{r-1,t\}} \binom{t}{j} \\
    &\quad \cdot \prod_{i=1}^{k+1} \Prob\left[\Prob[\Tcal_{i} < \Tcal_{i-1} | E, G_{[i-1]}] \in \iota(p_{i}) \big| E, S_{i-1} = w_i, G_{[i-2]} \in N(p_{[i-1]},w_{[i-2]})\right],
  \end{align*}
  which by Lemma \ref{lem:cdec} implies that
  \begin{align}
    &\Prob[G_{[k-1]} \in N(p_{[k]},w_{[k]}) \land \EbadB | E] \nonumber \\
    &\leq \hat{\delta} \left(\sum_{j=0}^{\min\{r-2,t\}} \binom{t}{j} + \sum_{j=0}^{\min\{r-1,t\}} \binom{t}{j}\right) \label{eq:nodeprobfull1} \\
    &\quad \cdot \prod_{i=1}^{k} \Prob\left[\Prob[\Tcal_{i} < \Tcal_{i-1} | E, G_{[i-1]}] \in \iota(p_i) \big| E, S_{i-1} = w_i, G_{[i-2]} \in N(p_{[i-1]},w_{[i-1]})\right]. \nonumber
  \end{align}
  To complete the proof, we need only consider two cases on the relationship between $t$ and $r$.  First, if $t \leq r-2$, then Pascal's rule implies that
  \begin{align*}
    \sum_{j=0}^{\min\{r-2,t\}} \binom{t}{j} + \sum_{j=0}^{\min\{r-1,t\}} \binom{t}{j} &= 2\sum_{j=0}^{t} \binom{t}{j} \\
    &= \binom{t}{t} + \binom{t}{0} + \sum_{j=1}^t \left(\binom{t}{j} + \binom{t}{j-1}\right) \\
    &= \binom{t+1}{t+1} + \binom{t+1}{0} + \sum_{j=1}^t \binom{t+1}{j} \\
    &= \sum_{j=0}^{t+1} \binom{t+1}{j} = \sum_{j=0}^{h(N_{p_{[k]},w_{[k]}})}  \binom{h(N_{p_{[k]},w_{[k]}})}{j}.
  \end{align*}
  Since $t \leq r-2$, it follows that $h(N_{p_{[k]},w_{[k]}}) = t+1 \leq r-1 = \smax-w_{k}-1$, which combined with \eqref{eq:nodeprobfull1} proves the result in this case.  Second, if $t > r-2$, then similarly
  \begin{align*}
    \sum_{j=0}^{\min\{r-2,t\}} \binom{t}{j} + \sum_{\hat{j}=0}^{\min\{r-1,t\}} \binom{t}{\hat{j}} &= \sum_{j=0}^{r-2} \binom{t}{j} + \sum_{\hat{j}=0}^{r-1} \binom{t}{\hat{j}} \\
    &= \binom{t}{0} + \sum_{j=1}^{r-1} \left(\binom{t}{j} + \binom{t}{j-1}\right) \\
    &= \binom{t+1}{0} + \sum_{j=1}^{r-1} \binom{t+1}{j} \\
    &= \sum_{j=0}^{r-1} \binom{t+1}{j} = \sum_{j=0}^{\smax-w_{k}-1} \binom{h(N_{p_{[k]},w_{[k]}})}{j}.
  \end{align*}
  Since $t > r-2$, $h(N_{p_{[k]},w_{[k]}}) = t+1 > r-1 = \smax-w_{k-1}-1$, which combined with \eqref{eq:nodeprobfull1} proves the result for this case as well. \qed
\eproof

We now prove our first main result of this section.

\begin{corollary} \label{coro:probbounded}
  Let Assumption \ref{assum:eventE} hold, let $\delta \in (0,1)$, and let $\hat{\delta}$ be computed as in \eqref{eq:hatdelta}, i.e.
  \bequationNN
    \hat{\delta} := \frac{\delta}{\sum_{j=0}^{\min\{\smax-1,\kmax\}} \binom{\kmax}{j}}.
  \eequationNN
  Then,
  \bequationNN
    \Prob\left[\sum_{i=0}^{\kmax} \Prob[\Tcal_i < \Tcal_{i-1} | E, G_{[i-1]}] \leq \ell(s_{\max},\hat{\delta})+1 \Bigg| E \right] \geq 1-\delta.
  \eequationNN
\end{corollary}
\bproof
  By the definitions of $\Lgood$ and $\Lbad$, $h(N(p_0,0)) \leq \kmax$. Therefore, by Lemma \ref{lem:nodeprobfull}, for any $B \in \N{}_{>0}$,
  \bequationNN
    \Prob[\EbadB | E] = \Prob[x_0 \in N(p_0,0) \land \EbadB | E] \nonumber \\
    \leq \hat{\delta} \sum_{j=0}^{\min\{\smax-1,\kmax\}} \binom{\kmax}{j} = \delta.
  \eequationNN
  Therefore, by the definition of $\EbadB$, it follows that
  \bequationNN
    \Prob\left[\sum_{i=0}^{\kmax} \Prob[\Tcal_i < \Tcal_{i-1} | E, G_{[i-1]}] \leq \ell(s_{\max},\hat{\delta}) + \frac{\kmax+1}{B}+1 \Bigg| E \right] \geq 1-\delta.
  \eequationNN
  
  Next, consider the sequence of events $E_{\text{good},B}$ defined by:
  \bequationNN
    \sum_{i=0}^{\kmax} \Prob[\Tcal_i < \Tcal_{i-1} | E, G_{[i-1]}] \leq \ell(s_{\max},\hat{\delta}) + \frac{\kmax+1}{B}+1,
  \eequationNN
  for all $B \in \N{}_{>0}$. It follows that
  \bequationNN
    E_{\text{good},B} \supseteq E_{\text{good},B+1},
  \eequationNN
  for all $B \in \N{}_{>0}$, so that $E_{\text{good},B}$ is a decreasing sequence of events. Therefore,
  \begin{align*}
    &\Prob\left[\sum_{i=0}^{\kmax} \Prob[\Tcal_i < \Tcal_{i-1} | E, G_{[i-1]}] \leq \ell(s_{\max},\hat{\delta}) +1 \Bigg| E \right] \\
    &= \Prob\left[\lim_{B \rightarrow \infty} \right(\sum_{i=0}^{\kmax} \Prob[\Tcal_i < \Tcal_{i-1} | E, G_{[i-1]}] \leq \ell(s_{\max},\hat{\delta}) + \frac{\kmax+1}{B}+1\left) \Bigg| E \right] \\
    &= \lim_{B \rightarrow \infty} \Prob\left[\sum_{i=0}^{\kmax} \Prob[\Tcal_i < \Tcal_{i-1} | E, G_{[i-1]}] \leq \ell(s_{\max},\hat{\delta}) + \frac{\kmax+1}{B}+1 \Bigg| E \right] \\
    &\leq 1-\delta.
  \end{align*}
  \qed
\eproof

Now, we are prepared to prove Lemma \ref{lem:Eksumlsmax}. For convenience, we restate the lemma here.

\begin{lemma} \label{lem:EksumlsmaxAppendix}
    Let Assumption \ref{assum:eventE} hold. Then,
    \bequationNN
        \Prob\left[\sum_{k=0}^{k_{\max}} \Prob [\Ek3 | E, \mathcal{F}_k] \leq \ell(s_{\max},\hat{\delta}) + 1 \Bigg| E\right] \geq 1-\delta,
    \eequationNN
    where $\hat{\delta}$ is defined in \eqref{eq:hatdelta}.
\end{lemma}

\begin{proof}
    We note that, for any $k \in [\kmax]$, by the defintion of $\Ek3$, the event $\Tcal_k < \Tcal_{k-1}$ must occur whenever $\Ek3$ occurs. Therefore, for any $k \in [\kmax]$,
    \bequationNN
        \Prob[\Tcal_k < \Tcal_{k-1} | E, \Fcal_k] \geq \Prob[\Ek3 | E, \Fcal_k].
    \eequationNN
    The result then follows directly by Corollary \ref{coro:probbounded}. \qed
\end{proof}

Now, we turn our focus on proving Lemma \ref{lem:Ktaulsmax}. We recall the random index set $\Kcal_{\tau}$ defined in \eqref{eq:Ktau} and let a realization of this set be denoted by $\ktau$. For the reader's convenience, we repeat these definitions here:
\bequationNN
    \Kcal_{\tau} = \{k \in [\kmax] : \tcalktritrue < \Tcal_{k-1}\},
\eequationNN
and
\bequationNN
    \ktau := \{k \in [\kmax] : \tktritrue < \tau_{k-1}\}.
\eequationNN

Now, we state an important property about iterations, given a specific realization $g_{[k-1]}$ of $G_{[k-1]}$, at which the event $k \in \ktau$ occurs.

\blemma \label{lem:Etautrial}
    Let Assumptions \ref{assum:eventE} and \ref{assum:ptau} hold. Then,
    \bequation
        \Prob[\Tcal_k < \tau_{k-1} | E, g_{[k-1]}, k \in \ktau] \geq p_{\tau}.
    \eequation
\elemma

\bproof
    On any iteration where $\tktritrue < \tau_{k-1}$ occurs, it follows that $\tktritrue < \infty$, so
    \bequationNN
        \tktritrue = \frac{(1-\sigma)\|c_k\|_1}{\nabla f(x_k)^\top \dktrue + \max\{(\dktrue)^\top H_k \dktrue,0\}}
    \eequationNN
    and thus
    \bequationNN
        (1-\sigma)\|c_k\|_1 < (\nabla f(x_k)^\top \dktrue + \max\{(\dktrue)^\top H_k \dktrue,0\}) \tau_{k-1}.
    \eequationNN
    
    By the definition of $\tau_k$, if
    \bequationNN
        g_k^\top d_k + \max\{d_k^\top H_k d_k,0\} \geq \nabla f(x_k)^\top \dktrue + \max\{(\dktrue)^\top H_k \dktrue,0\}
    \eequationNN
    occurs on an iteration such that $\tktritrue < \tau_{k-1}$, then
    \bequationNN
        (1-\sigma)\|c_k\|_1 < (g_k^\top d_k + \max\{d_k^\top H_k d_k,0\}) \tau_{k-1}
    \eequationNN
    occurs as well so that $\tau_k < \tau_{k-1}$. Noting that the event $k \in \ktau$ is conditionally independent of $G_k$ given $E$ and $g_{[k-1]}$, it follows that
    \begin{align*}
        &\Prob[\Tcal_k < \tau_{k-1} | E, g_{[k-1]}, k \in \ktau] \\
        &\geq \Prob[G_k^\top D_k + \max\{D_k^\top H_k D_k,0\} \geq \nabla f(x_k)^\top \dktrue + \max\{(\dktrue)^\top H_k \dktrue,0\} | E, g_{[k-1]}, k \in \ktau] \\
        &= \Prob[G_k^\top D_k + \max\{D_k^\top H_k D_k,0\} \geq \nabla f(x_k)^\top \dktrue + \max\{(\dktrue)^\top H_k \dktrue,0\} | E, g_{[k-1]}] \\
        &\geq p_{\tau}.
    \end{align*} \qed
\eproof

The previous lemma guarantees that any iteration where $\tktritrue < \tau_{k-1}$ holds, there is at least $p_{\tau}$ probability of decreasing $\tau$ at iteration $k$. By the definition of $\tau_k$,
\bequation \label{eq:cardinality1}
    \Prob[\tktritrue < \tau_k | E, g_{[k-1]}, \tktritrue \geq \tau_{k-1}] = 0,
\eequation
so $\tktritrue < \tau_{k-1}$ must occur at any iteration where $\hat{\tau}_k < \tau_k$, where $\hat{\tau}_k$ is a realization of the random variable $\hat{\Tcal}_k$ defined in \eqref{eq:hattaudef}. Thus, we can obtain a bound on the number of iterations at which $\tktritrue < \tau_k$ by bounding the number of iterations at which $\tktritrue < \tau_{k-1}$. Now we prove a result relating $|\Kcal_{\tau}|$ to the probability of decreasing the merit paremeter at each iteration.

\blemma \label{lem:probktaudec}
    Let Assumptions \ref{assum:eventE} and \ref{assum:ptau} hold. Then,
    \bequation
        \sum_{k=0}^{\kmax} \Prob[\Tcal_k < \Tcal_{k-1} | E, \Fcal_k] \geq |\Kcal_{\tau}| p_{\tau}.
    \eequation
\elemma

\bproof
    We begin by considering any realization $g_{[\kmax]}$ which is measurable with respect to the filtration $\Fcal_{\kmax+1}$. Then, by Lemma \ref{lem:Etautrial}, for all $k \in [\kmax]$,
    \begin{align*}
        &\quad \ \Prob[\Tcal_k < \tau_{k-1} | E, g_{[k-1]}] \\
        &\geq \Prob[\Tcal_k < \tau_{k-1} \land k \in \ktau | E, g_{[k-1]}] \\
        &= \Prob[\Tcal_k < \tau_{k-1} | E, g_{[k-1]}, k \in \ktau] \Prob[k \in \ktau | E, g_{[k-1]}] \\
        &= \Prob[\Tcal_k < \tau_{k-1} | E, g_{[k-1]}, k \in \ktau] \Ical[k \in \ktau] \\
        &\geq \Ical[k \in \ktau] p_{\tau},
    \end{align*}
    where $\Ical[k \in \ktau]$ is the indicator function for the event $k \in \ktau$ and the second equality follows due to the fact that the event $k \in \ktau$ is deterministically known when conditioned on $g_{[k-1]}$. Summing this for all $k$,
    \bequationNN
        \sum_{k=0}^{\kmax} \Prob[\Tcal_k < \tau_{k-1} | E, g_{[k-1]}] \geq \sum_{k=0}^{\kmax} \Ical[k \in \ktau] p_{\tau} = |\ktau| p_{\tau}.
    \eequationNN
    
    Let $f_{G_{[\kmax]}}$ denote the probability density function of $G_k$. Then, since the above inequality holds \emph{deterministically} for any $g_{[\kmax]}$ which is measurable with respect to $\Fcal_{\kmax+1}$, by the law of total probability,
    \begin{align*}
        &\Prob\left[\sum_{k=0}^{\kmax} \Prob[\Tcal_k < \Tcal_{k-1} | E, \Fcal_{k-1}] \geq |\Kcal_{\tau}| p_{\tau} \ \Bigg| E\right] \\
        &=\int_{g_{[\kmax]} \in \Fcal_{\kmax+1}} \Prob\left[\sum_{k=0}^{\kmax} \Prob[\Tcal_k < \tau_{k-1} | E, g_{[k-1]}] \geq |\ktau| p_{\tau} \ \Big| E, g_{[\kmax]}\right] f_{G_{[\kmax]}}(g_{[k-1]}) dg \\
        &= \int_{g_{[\kmax]} \in \Fcal_{\kmax+1}} 1 \cdot f_{G_{[\kmax]}}(g_{[k-1]}) dg = 1.
    \end{align*}
    Therefore, the desired result holds as well. \qed
\eproof

Now, we restate and prove Lemma \ref{lem:Ktaulsmax}.

\begin{lemma} \label{lem:KtaulsmaxAppendix}
    Let Assumptions \ref{assum:eventE} and \ref{assum:ptau} hold. Let $\mathcal{K}_{\tau}$ be defined in \eqref{eq:Ktau}. Then, for any $\delta \in (0,1)$, it follows that
    \bequationNN
        \Prob\left[|\mathcal{K}_{\tau}| \leq \left\lceil \frac{\ell(s_{\max},\hat{\delta})+1}{p_{\tau}}\right\rceil \Bigg| E\right] \geq 1-\delta.
    \eequationNN
\end{lemma}

\begin{proof}
    The proof follows directly by combining the results of Corollary \ref{coro:probbounded} and Lemma \ref{lem:probktaudec}. \qed
\end{proof}

Finally, we conclude this appendix by showing that the order notation result in \eqref{eq.like_sg} and \eqref{eq.new_terms} holds.

\blemma \label{lem:Orderlsd}
    Let $\delta \in (0,1)$, $\hdelta$ be defined in \eqref{eq:hatdelta}, and $\ell(\smax,\hdelta)$ be defined in \eqref{eq:lsd}. Then,
    \bequationNN
        \ell(\smax,\hdelta) = \Ocal\left(\smax\log(\kmax) + \log(1/\delta)\right).
    \eequationNN
\elemma
    
\bproof
    We start by noting that since $\smax \leq \kmax+1$,
    \begin{align*}
        \sum_{j=0}^{\min\{\smax-1,\kmax\}} \binom{\kmax}{j}
        &= \sum_{j=0}^{\smax-1} \frac{(\kmax)!}{j!(\kmax-j)!} \\
        &\leq \sum_{j=0}^{\smax-1} \frac{(\kmax)!}{(\kmax-j)!} \\
        &= 1+\sum_{j=1}^{\smax-1} \prod_{i=\kmax+1-j}^{\kmax} i \\
        &\leq 1+\sum_{j=1}^{\smax-1} (\kmax)^j \\
        &\leq 1+(\smax-2) (\kmax)^{\smax-1} \\
        &\leq (\smax-1) (\kmax)^{\smax-1}.
    \end{align*}
    Then, by the definitions of $\ell(\smax,\hdelta)$ and $\hdelta$,
    \begin{align*}
        \ell(\smax,\hdelta) &= \Ocal\left(\smax + \log(1/\hdelta)\right) \\
        &= \Ocal\left(\smax + \log(\smax-1) + (\smax-1)\log(\kmax) + \log(1/\delta)\right) \\
        &= \Ocal\left(\smax\log(\kmax) + \log(1/\delta)\right).
    \end{align*}
    \qed
\eproof

\iffalse
\newpage 
All old stuff below here:

Update 7/8:

We can define a node in the graph in terms of a set of realizations with the following properties. We say that $g_0,\dots,g_{k-1} \in N([p_0,\dots,p_k],[s_0,\dots,s_{k-1}])$ if
\begin{align*}
    &\Prob[\Tcal_k < \tau_{k-1} | E, g_0,\dots,g_{k-1}] = p_k, \\
    &S_{k-1} := \sum_{i=0}^{k-1} \Ical[\tau_i < \tau_{i-1}] = s_{k-1}, \\
    &g_0,\dots,g_{k-2} \in N([p_0,\dots,p_{k-1}],[s_0,\dots,s_{k-2}]).
\end{align*}
For the $i$-th node at depth $k$, we adopt the notation $N_{k,i} = N([p_{0,i},\dots,p_{k,i}],[s_{0,i},\dots,s_{k-1,i}])$.
We denote by $P(N_k)$, the parent node $N_{k-1}$. Similarly, we denote the set of children of node $N_k$ by $C(N_k)$.

Simple things:
Using this definition, the probability of reaching any particular node $N_k$ is given by (where we abuse notation a bit and let $\Prob[\bar{G}_{k-1} \in N_k | E] = \Prob[G_0,\dots,G_{k-1} \in N_k | E]$:
\begin{align*}
    &\Prob[\bar{G}_{k-1} \in N_k | E] \\
    &= \Prob[\Prob[\Tcal_k < \tau_{k-1} | E, \bar{G}_{k-1}] = p_k \cap S_{k-1} = s_{k-1} \cap \bar{G}_{k-2} \in N_{k-1} | E] \\
    &= \Prob[\Prob[\Tcal_k < \tau_{k-1} | E, \bar{G}_{k-1}] = p_k | S_{k-1} = s_{k-1}, \bar{G}_{k-2} \in N_{k-1}, E] \Prob[S_{k-1} = s_{k-1} \cap \bar{G}_{k-2} \in N_{k-1} | E] \\
    &= \Prob[\Prob[\Tcal_k < \tau_{k-1} | E, \bar{G}_{k-1}] = p_k | S_{k-1} = s_{k-1}, \bar{G}_{k-2} \in N_{k-1}, E] \Prob[S_{k-1} = s_{k-1} | \bar{G}_{k-2} \in N_{k-1}, E] \Prob[\bar{G}_{k-2} \in N_{k-1}, E],
\end{align*}
so we can unroll this recursively. It's not pretty though...

Let $\Lbad$ denote the set of nodes of the tree that satisfy:
\begin{align*}
    \sum_{i=0}^{k} p_i &\geq \ell(s_{\max},\delta), \\
    \sum_{i=0}^{k-1} p_i &< \ell(s_{\max},\delta), \\
    s_{k-1} &< s_{\max}.
\end{align*}
We want to find $\ell(s_{\max},\delta)$ such that the probability of a realization has a node in $\Lbad$ is no more than $\delta$.

For any realization, $g_0,\dots,g_{k-1}$ for some $k \in \{0,\dots,k_{\max}\}$, they belong to the event $E_{bad}$ if
\bequationNN
    \sum_{i=0}^k \Prob[\Tcal_i < \tau_{i-1} | E, g_0,\dots,g_{i-1}] \geq \ell(s_{\max},\delta)
\eequationNN
and $s_{k-1} < s_{\max}$ holds. Want to bound $\Prob[E_{bad} | E]$. Can bound it by:
\bequationNN
    \Prob[E_{bad} | E] =  \sum_{i \in \Lbad} \Prob[N_i | E]
\eequationNN

Let $\Ncal_k$ denote the set of all nodes with depth $k$.

\bequationNN
    \Prob[E_{bad} | E] = \sum_{i \in \Ncal_1} \Prob[E_{bad} | E, g_0 \in N_i] \Prob[g_0 \in N_i | E] = \sum_{i \in \Ncal_1}
    \Prob[g_0 \in N_i | E]
    \sum_{j \in C(N_i)}\Prob[E_{bad} | E, g_0 \in N_i, (g_0,g_1) \in N_j] \Prob[(g_0,g_1) \in N_j | E, g_0 \in N_i] 
\eequationNN


Old stuff:

In this section, we prove Lemma \ref{lem:Eksumlsmax} and Lemma \ref{lem:Ktaulsmax} under Assumptions \ref{assum:fcsmooth}, \ref{assum:eventE}, and \ref{assum:ptau}. We focus on proving Lemma \ref{lem:Eksumlsmax} because techniques derived for this case can be easily extended to proving Lemma \ref{lem:Ktaulsmax} under Assumption \ref{assum:ptau}. To this end, we introduce a set of Bernoulli random variables which model the properties of $\tau_k$ decreasing in relation to the maximum number of $\tau_k$ decreases, $s_{\max}$. We derive high probability bounds for these random variables and show that these bounds hold for the $\tau_k$ sequence generated by Algorithm \ref{alg:ssqp}, which is used to prove Lemma \ref{lem:Eksumlsmax} and Lemma \ref{lem:Ktaulsmax}.

For the remainder of this appendix, let $Z_k$ for $k \in \{0,\dotsc,k_{\max}\}$ be Bernoulli random variables which satisfy
\bequation \label{eq:zkdef}
  \baligned
    \Prob\left[Z_k = 1 \Bigg| \sum_{i=0}^{k-1} Z_i < s_{\max}\right] &= p_k \\ \text{and}\ \ 
    \Prob\left[Z_k = 1 \Bigg| \sum_{i=0}^{k-1} Z_i \geq s_{\max}\right] &= 0,
  \ealigned
\eequation
where $s_{\max}$ is defined in Assumption \ref{assum:eventE} and $p_k \in [0,1]$ for all $k \in \{0,\dotsc,k_{\max}\}$. We begin by proving a simple result relating to the summation of these probabilities.
\begin{lemma} \label{lem:simple1}
    Let $Z_k$ be defined as in \eqref{eq:zkdef}.
    Then, for any $j \in \{s_{\max}, \dotsc, k_{\max}\}$,
    \bequation \label{eq:simple1}
        \Prob\left[ \sum_{k=0}^{k_{\max}} \Prob\left[Z_k = 1 \Bigg| \sum_{i=0}^{k-1} Z_i\right] \leq \sum_{k=0}^{j-1} p_k \right] \geq \Prob\left[\sum_{k=0}^{j-1} Z_k = s_{\max} \right].
    \eequation
\end{lemma}

\begin{proof}
    Let $E_j$ be the event that $\sum_{k=0}^{j-1} Z_k = s_{\max}$. Then, by the definition of $Z_k$,
    \bequationNN
        \Prob\left[Z_k = 1 \Bigg| \sum_{i=0}^{k-1} Z_i, E_j \right] = 0, \text{ for all $k \geq j$}.
    \eequationNN
    Therefore,
    \begin{align*}
        &\sum_{k=0}^{k_{\max}} \Prob\left[Z_k = 1 \Bigg| \sum_{i=0}^{k-1} Z_i, E_j\right] \\
        &= \sum_{k=0}^{j-1} \Prob\left[Z_k = 1 \Bigg| \sum_{i=0}^{k-1} Z_i, E_j\right] + \sum_{k=j}^{k_{\max}} \Prob\left[Z_k = 1 \Bigg| \sum_{i=0}^{k-1} Z_i, E_j\right] \\
        &\leq \sum_{k=0}^{j-1} p_k + \sum_{k=j}^{k_{\max}} 0 = \sum_{k=0}^{j-1} p_k.
    \end{align*}
    
    Then, by the law of total probability,
    \begin{align*}
        &\Prob\left[ \sum_{k=0}^{k_{\max}} \Prob\left[Z_k = 1 \Bigg| \sum_{i=0}^{k-1} Z_i\right] \leq \sum_{k=0}^{j-1} p_k \right] \\
        &= \Prob\left[ \sum_{k=0}^{k_{\max}} \Prob\left[Z_k = 1 \Bigg| \sum_{i=0}^{k-1} Z_i\right] \leq \sum_{k=0}^{j-1} p_k \Bigg| E_j \right] \Prob[E_j] \\
        &\quad+ \Prob\left[ \sum_{k=0}^{k_{\max}} \Prob\left[Z_k = 1 \Bigg| \sum_{i=0}^{k-1} Z_i\right] \leq \sum_{k=0}^{j-1} p_k \Bigg| E_j^c \right] \Prob[E_j^c] \\
        &\geq 1 \Prob[E_j] = \Prob[E_j],
    \end{align*}
    which completes the proof.
\end{proof}

Recalling that we wish to prove a bound on the sum of these probabilities in high probability (as our goal is to prove \eqref{eq:Ek3lsmax}), it's clear that a lower bound on the right side of \eqref{eq:simple1} is needed. By the law of total probability and the definition of $Z_k$,
\bequationNN
    \Prob\left[\sum_{k=0}^{\ell} Z_k = s_{\max} \right] = 1 - \Prob\left[\sum_{k=0}^{\ell} Z_k < s_{\max} \right],
\eequationNN
so that we can target the right hand side of this equation instead.
\begin{lemma} \label{lem:simple2}
    Let $j \in \{s_{\max}-1,\dotsc,k_{\max}\}$, let $Z_0,\dotsc,Z_j$ be defined by \eqref{eq:zkdef}, and let $\hat{Z}_0,\dotsc,\hat{Z}_j$ be independent Bernoulli random variables with $\Prob[\hat{Z}_k = 1] = p_k$. Then,
    \bequationNN
        \Prob\left[\sum_{k=0}^j Z_k < s_{\max} \right] = \Prob\left[\sum_{k=0}^{j} \hat{Z}_k < s_{\max} \right].
    \eequationNN
\end{lemma}

\begin{proof}
    For all $k \in \{0,\dotsc,j\}$, let $\hat{z}_k$ be a realization of the random variable $\hat{Z}_k$. Then, for all $k \in \{0,\dotsc,j\}$, let
    \bequationNN 
        \bar{z}_k := \bcases
        1 & \textrm{when } \hat{z}_k = 1 \textrm{ and } \sum_{i=0}^{k-1} \bar{z}_i < s_{\max} \\
        0 & \textrm{otherwise},
        \ecases
    \eequationNN
    and let $\bar{Z}_k$ denote the Bernoulli random variable of which $\bar{z}_k$ is a realization. By the definition of $\hat{Z}_k$
    and the definition of $\bar{Z}_k$, it follows that
    \begin{align*}
        \Prob\left[\bar{Z}_k = 1 \Bigg| \sum_{i=0}^{k-1} \bar{Z}_i < s_{\max}\right] &= p_k \\
        \textrm{and } \Prob\left[\bar{Z}_k = 1 \Bigg| \sum_{i=0}^{k-1} \bar{Z}_i \geq s_{\max}\right] &= 0
    \end{align*}
    
    Therefore, by \eqref{eq:zkdef}, $\bar{Z}_0, \dotsc, \bar{Z}_j$ are equivalent in distribution to $Z_0, \dotsc, Z_j$. Now, by the definition of $\bar{Z}_k$, the event $\sum_{k=0}^j \hat{Z}_k < s_{\max}$ occurs if and only if the event $\sum_{k=0}^j \bar{Z}_k < s_{\max}$ occurs as well. Thus,
    \bequationNN
        \Prob\left[\sum_{k=0}^j \hat{Z}_k < s_{\max}\right] = \Prob\left[ \sum_{k=0}^j \bar{Z}_k < s_{\max}\right] = \Prob\left[ \sum_{k=0}^j Z_k < s_{\max}\right],
    \eequationNN
    where the last equality holds because 
    $\bar{Z}_0, \dotsc, \bar{Z}_j$ and $Z_0, \dotsc, Z_j$ are equivalent in distribution.
\end{proof}

Now, since a relationship between $Z_k$ and a set of independent Bernoulli random variables has been established, we can utilize Chernoff's bound, as we show in the following lemma.

\blemma\label{lem:chernoff}
  For any $k \in \N{}$, let $\{Y_0,\dots,Y_k\}$ be independent Bernoulli random variables.  Then, for any $s \in \N{}_{>0}$ and $\delta \in (0,1)$, it follows that
  \bequation \label{eq:chernoffeq1}
    \mu := \sum_{j=0}^k \P[Y_j = 1] \geq \ell(s,\delta)\ \ \implies \ \ \P\left[\sum_{j=0}^k Y_j \leq s\right] \leq \delta,
  \eequation
  where $\ell(s,\delta)$ is defined in \eqref{eq:lsd}.
\elemma
\bproof
  By the multiplicative form of Chernoff's bound, it follows for $\rho := 1 - s/\mu$ (which is in the interval $(0,1)$ by (\ref{eq:chernoffeq1})) that
  \bequationNN
    \P\left[\sum_{j=0}^{k} Y_j \leq s \right] \leq e^{-\frac{\mu \rho^2}{2}} = e^{-\frac{\mu (1-s/\mu)^2}{2}}.
  \eequationNN
  Hence, to prove the result, all that remains is to show that $e^{-\frac{\mu (1-s/\mu)^2}{2}} \leq \delta$, i.e.,
  \bequationNN
    -\frac{\mu(1-s/\mu)^2}{2} \leq \log(\delta)
  \eequationNN
  Using $\log(\delta) = -\log(1/\delta)$, this inequality is equivalent to
  \bequationNN
    0 \leq \frac{\mu(1-s/\mu)^2}{2} - \log(1/\delta) = \frac{(\mu - s)^2}{2\mu} - \log(1/\delta),
  \eequationNN
  which holds if and only if $\mu^2 - 2\mu (s+\log(1/\delta)) + s^2 \geq 0$.  Viewing the left-hand side of this inequality as a convex quadratic function in $\mu$, one finds that the inequality holds as long as $\mu$ is greater than or equal to the positive root of the quadratic, i.e.,
  \bequationNN
    \baligned
      \mu
        &\geq s + \log(1/\delta) + \sqrt{(s+\log(1/\delta))^2 - s^2} \\
        &= s + \log(1/\delta) + \sqrt{\log(1/\delta)^2 + 2s\log(1/\delta)}.
    \ealigned
  \eequationNN
  Since this holds under assumption in the lemma, the result is proved.
\eproof

Now, we can combine Lemma \ref{lem:simple1}, \ref{lem:simple2} and \ref{lem:chernoff} to provide a bound reminiscent of which is similar in form to \eqref{eq:Ek3lsmax}.

\begin{lemma} \label{lem:simple3}
    Let $s_{\max} \in \{1,\dotsc,k_{\max}\}$ and $\delta \in (0,1)$.
    For all $k \in \{0,\dotsc,k_{\max}\}$, let $Z_k$ be Bernoulli random variables defined by \eqref{eq:zkdef}. Then,
    \bequation
        \Prob\left[\sum_{k=0}^{k_{\max}} \Prob \left[Y_k = 1 \Bigg| \sum_{i=0}^{k-1} Z_i \right] \leq \ell(s_{\max},\delta) + 1\right] \geq 1 - \delta,
    \eequation
    where $\ell(s_{\max},\delta)$ is defined in \eqref{eq:lsd}.
\end{lemma}

\begin{proof}
    Let $\sum_{k=0}^{k_{\max}} p_k \leq \ell(s_{\max},\delta) + 1$. Then, by the definition of $Z_k$, it is clear that
    \bequationNN
        \sum_{k=0}^{k_{\max}} \Prob \left[Z_k = 1 \Bigg| \sum_{i=0}^{k-1} Z_i \right] \leq \ell(s_{\max},\delta) + 1
    \eequationNN
    holds deterministically, so the result is trivial in this case. Thus, for the remainder of the proof, we assume that $\sum_{k=0}^{k_{\max}} p_k > \ell(s_{\max},\delta) + 1$.
    
    Now, let $k_{s_{\max},\delta}$ be the minimum integer such that
    \bequationNN
        \sum_{k=0}^{k_{s_{\max},\delta}} p_k \geq \ell(s_{\max},\delta).
    \eequationNN
    Let $\hat{Z}_0,\dotsc,\hat{Z}_{k_{s_{\max},\delta}}$ be independent Bernoulli random variables with $\Prob[\hat{Y}_k = 1] = p_k$. Then, by Lemma \ref{lem:simple2} and Lemma \ref{lem:chernoff},
    \bequationNN
        \Prob\left[\sum_{k=0}^{k_{s_{\max},\delta}} Z_k < s_{\max}\right] = \Prob\left[\sum_{k=0}^{k_{s_{\max},\delta}} \hat{Z}_k < s_{\max}\right] \leq \Prob\left[\sum_{k=0}^{k_{s_{\max},\delta}} \hat{Z}_k \leq s_{\max}\right] \leq \delta.
    \eequationNN
    Finally, by Lemma \ref{lem:simple1},
    \begin{align*}
        \Prob\left[ \sum_{k=0}^{k_{\max}} \Prob\left[Z_k = 1 \Bigg| \sum_{i=0}^{k-1} Z_i\right] \leq \sum_{k=0}^{k_{s_{\max},\delta}} p_k \right] &\geq \Prob\left[\sum_{k=0}^{k_{s_{\max},\delta}} Z_k = s_{\max} \right] \\
        &= 1 - \Prob\left[\sum_{k=0}^{k_{s_{\max},\delta}} Z_k < s_{\max} \right] \\
        &\geq 1 - \delta.
    \end{align*}
    The result follows by noting that $\sum_{k=0}^{k_{s_{\max},\delta}} p_k \leq \ell(s_{\max},\delta) + 1$.
\end{proof}

Now, we are prepared to prove Lemma \ref{lem:Eksumlsmax}. For convenience, we restate the lemma here.

\begin{lemma} \label{lem:EksumlsmaxAppendix}
    Let Assumption \ref{assum:eventE} hold. Then,
    \bequationNN
        \Prob\left[\sum_{k=0}^{k_{\max}} \Prob [E_{k,3} | E, \mathcal{F}_k] \leq \ell(s_{\max},\delta) + 1 \Bigg| E\right] \geq 1-\delta.
    \eequationNN
\end{lemma}

\begin{proof}
    Let $Z_k$ be the indicator of the event $E_{k,3}$ and let \\$P_k = \Prob[Z_k=1| E, \mathcal{F}_k, S_{k-1} < s_{\max}]$ and let $p_k \in [0,1]$ for all $k \in \{0,\dotsc,k_{\max}\}$. Then, by the definition of $s_{\max}$ in Assumption \ref{assum:eventE} and Lemma \ref{lem:simple3}, it follows that
\bequationNN
    \Prob\Bigg[\sum_{k=0}^{k_{\max}} \Prob[Z_k=1|E,\mathcal{F}_k] \leq \ell(s_{\max},\delta) + 1 \Bigg| E,\left\{P_0, \dotsc, P_{k_{\max}}\right\}
    = \left\{p_0,\dotsc,p_{k_{\max}}\right\}\Bigg] \geq 1-\delta,
\eequationNN
holds for any $\bar{p} = \{p_0,\dotsc,p_{k_{\max}}\}$ which is measurable with respect to the filtration $\mathcal{F}_{k_{\max}}$. Therefore, by the law of total probability
\begin{align*}
    &\Prob\left[\sum_{k=0}^{k_{\max}} \Prob[Z_k = 1| E,\mathcal{F}_k] \leq \ell(s_{\max},\delta) + 1 \Bigg| E\right] \\
    &=\int_{p \in [0,1]^{k_{\max} + 1}} \Prob\Bigg[\sum_{k=0}^{k_{\max}} \Prob[Z_k|E,\mathcal{F}_k] \leq \ell(s_{\max},\delta) + 1 \\
    &\quad\quad\quad\quad\quad\quad\quad\quad\quad \Bigg| E, \left\{P_0, \dotsc, P_{k_{\max}}\right\} 
    = \left\{p_0,\dotsc,p_{k_{\max}}\right\}\Bigg] f_{P}(p) dp \\
    &\geq (1 - \delta) \int_{p \in [0,1]^{k_{\max} + 1}} f_{P}(p) dp = 1 - \delta,
\end{align*}
where $f_P(p)$ is the probability density function of the random variable $P$.
\end{proof}

Now, we turn our focus on proving Lemma \ref{lem:Ktaulsmax}.

\blemma \label{lem:Etautrial}
    Let Assumptions \ref{assum:eventE} and \ref{assum:ptau} hold. Then,
    \bequation
        \Prob[\Tcal_k < \tau_{k-1} | E, \mathcal{F}_k, \tktritrue < \tau_{k-1}] \geq p_{\tau}.
    \eequation
\elemma

\bproof
    On any iteration where $\tktritrue < \tau_{k-1}$ occurs, it follows that $\tktritrue < \infty$, so
    \bequationNN
        \tktritrue = \frac{(1-\sigma)\|c_k\|_1}{\nabla f(x_k)^\top \dktrue + \max\{(\dktrue)^\top H_k \dktrue,0\}}
    \eequationNN
    and thus
    \bequationNN
        (1-\sigma)\|c_k\|_1 < (\nabla f(x_k)^\top \dktrue + \max\{(\dktrue)^\top H_k \dktrue,0\}) \tau_{k-1}.
    \eequationNN
    
    By the definition of $\tau_k$, if
    \bequationNN
        g_k^\top d_k + \max\{d_k^\top H_k d_k,0\} \geq \nabla f(x_k)^\top \dktrue + \max\{(\dktrue)^\top H_k \dktrue,0\}
    \eequationNN
    occurs on an iteration such that $\tktritrue < \tau_{k-1}$, then
    \bequationNN
        (1-\sigma)\|c_k\|_1 < (g_k^\top d_k + \max\{d_k^\top H_k d_k,0\}) \tau_{k-1}
    \eequationNN
    occurs as well so that $\tau_k < \tau_{k-1}$. Noting that $\tktritrue < \tau_{k-1}$ is conditionally independent of $G_k$ given $E$ and $\mathcal{F}_k$, it follows that
    \begin{align*}
        &\Prob[\Tcal_k < \tau_{k-1} | E, \mathcal{F}_k, \tktritrue < \tau_{k-1}] \\
        &\geq \Prob[G_k^\top D_k + \max\{D_k^\top H_k D_k,0\} \geq \nabla f(x_k)^\top \dktrue + \max\{(\dktrue)^\top H_k \dktrue,0\} | E, \mathcal{F}_k, \tktritrue < \tau_{k-1}] \\
        &= \Prob[G_k^\top D_k + \max\{D_k^\top H_k D_k,0\} \geq \nabla f(x_k)^\top \dktrue + \max\{(\dktrue)^\top H_k \dktrue,0\} | E, \mathcal{F}_k] \\
        &\geq p_{\tau}.
    \end{align*}
\eproof

The previous lemma guarantees that any iteration where $\tktritrue < \tau_{k-1}$ holds, there is at least $p_{\tau}$ probability of decreasing $\tau$ at iteration $k$. By the definition of $\tau_k$,
\bequation \label{eq:cardinality1}
    \Prob[\tktritrue < \tau_k | E, g_{[k-1]}, \tktritrue \geq \tau_{k-1}] = 0,
\eequation
so $\tktritrue < \tau_{k-1}$ must occur at any iteration where $\hat{\tau}_k < \tau_k$. Thus, we can obtain a bound on the number of ``bad" iterations by bounding the number of iterations at which $\tktritrue < \tau_{k-1}$. We derive this bound in the following lemma, where we prove Lemma \ref{lem:Ktaulsmax}. For convenience, we restate the lemma here.

\begin{lemma} \label{lem:KtaulsmaxAppendix}
    Let Assumptions \ref{assum:eventE} and \ref{assum:ptau} hold. Let $\mathcal{K}_{\tau} = \{k : \tktritrue < \tau_{k-1} \}$. Then,
    \bequationNN
        \Prob\left[|\mathcal{K}_{\tau}| \leq \left\lceil \frac{\ell(s_{\max},\delta)+1}{p_{\tau}}\right\rceil \Bigg| E\right] \geq 1-\delta.
    \eequationNN
\end{lemma}

\begin{proof}
    Let $Z_k$ be the indicator of the event that $\Tcal_k < \tau_{k-1}$ and let $P_k = \Prob[Z_k = 1 | \mathcal{F}_k, E, S_{k-1} < s_{\max}]$. Then, by the definition of $s_{\max}$ and Lemma \ref{lem:simple3}, it follows that
    \bequationNN
        \Prob\Bigg[\sum_{k=0}^{k_{\max}} \Prob[Z_k=1|E,\mathcal{F}_k] \leq \ell(s_{\max},\delta) + 1 \Bigg| E, \left\{P_0, \dotsc, P_{k_{\max}}\right\}
        = \left\{p_0,\dotsc,p_{k_{\max}}\right\}\Bigg] \geq 1-\delta,
    \eequationNN
    holds for any $p = \{p_0,\dots,p_{k_{\max}}\}$ which is measurable with respect to the filtration $\mathcal{F}_{k_{\max}}$. Therefore by the law of total probability,
    \begin{align*}
        &\Prob\left[\sum_{k=0}^{k_{\max}} \Prob[\Tcal_k < \tau_{k-1}| E,\mathcal{F}_k] \leq \ell(s_{\max},\delta) + 1 \Bigg| E\right] \\
        &=\int_{p \in [0,1]^{k_{\max} + 1}} \Prob\Bigg[\sum_{k=0}^{k_{\max}} \Prob[Z_k|E,\mathcal{F}_k] \leq \ell(s_{\max},\delta) + 1\\
        &\quad\quad\quad\quad\quad\quad\quad\quad\quad \Bigg| E, \left\{P_0, \dotsc, P_{k_{\max}}\right\} 
        = \left\{p_0,\dotsc,p_{k_{\max}}\right\}\Bigg] f_P(p) dp \\
        &\geq (1 - \delta) \int_{p \in [0,1]^{k_{\max} + 1}} f_{P}(p) dp = 1 - \delta,
    \end{align*}
    where $f_P$ is the probability density function of the random variable $P$.
    
    Now, recall that $\Tcal_k < \tau_{k-1}$ is conditionally independent of $\tktritrue < \tau_{k-1}$ given $\Fcal_k$ and $E$. Then, by Lemma \ref{lem:Etautrial},
    \bequationNN
        \sum_{k=0}^{k_{\max}} \Prob\left[\Tcal_k < \tau_{k-1}| E, \Fcal_k \right] \geq \sum_{k \in \Kcal_{\tau}} \Prob\left[\Tcal_k < \tau_{k-1}| E, \Fcal_k, \tktritrue < \tau_{k-1} \right] \geq |\Kcal_{\tau}| p_{\tau}.
    \eequationNN
    
    Combining the above two inequalities, it follows that
    \bequationNN
        \Prob[ |\Kcal_{\tau}| p_{\tau} \leq \ell(s_{\max},\delta)+1 | E] \geq 1-\delta,
    \eequationNN
    and thus,
    \bequationNN
        \Prob\left[|\mathcal{K}_{\tau}| \leq \left\lceil \frac{\ell(s_{\max},\delta)+1}{p_{\tau}}\right\rceil \Bigg| E\right] \geq 1-\delta.
    \eequationNN
\end{proof}

\section{Proof of Proposition 3.16 of \cite{ABerahas_FECurtis_DPRobinson_BZhou_2021}}

We will prove this proposition by showing that the cardinality of the index set:
\bequationNN
    \Kcal_{\tau} := \{k : \tktritrue < \tau_{k-1}\},
\eequationNN
is finite with probability 1. By the definition of $\tau_k$, it follows that if $\tktritrue \geq \tau_{k-1}$, then $\tktritrue \geq \tau_k$. Therefore, if $\Kcal_\tau$ is finite, then $E_{\tau \gg 0}$ cannot occur.

We let $\Fcal_k$ denote our filtration at iteration $k$ (encodes the full history of our algorithm and allows us to condition on the past randomness). For the rest of the appendix, we adopt the notation $\Prob[\cdot|\Fcal_k] = \Prob_k[\cdot]$.

We begin by proving a relevant property about iterations such that $k \in \Kcal_{\tau}$.

\blemma \label{lem:tautrialextra}
    Let the assumptions of \cite{ABerahas_FECurtis_DPRobinson_BZhou_2021} hold.
    For all $k \in \N{}_{>0}$, let
    \bequationNN
        \Prob_k[G_k^\top D_k + \max\{D_k^\top H_k D_k,0\} \geq \nabla f(x_k)^\top \dktrue + \max\{(\dktrue)^\top H_k \dktrue,0\}] \geq p_{\tau}.
    \eequationNN
    Then,\footnote{FEC: What is $p_\tau$ here?  Is it supposed to be the same as $p$ above?}
    \bequation
        \Prob[\Tcal_k < \tau_{k-1} | \mathcal{F}_k, \tktritrue < \tau_{k-1}] \geq p_\tau.
    \eequation
\elemma

\bproof
  %\footnote{FEC: So I guess we're effectively saying here: ``Consider an iteration where $\tktritrue < \tau_{k-1}$,'' yes?}
   Consider an iteration $k$ such that $\tktritrue < \tau_{k-1}$. Then,  $\tktritrue < \infty$ and
    \bequationNN
        \tktritrue = \frac{(1-\sigma)\|c_k\|_1}{\nabla f(x_k)^\top \dktrue + \max\{(\dktrue)^\top H_k \dktrue,0\}}
    \eequationNN
    and thus
    \bequationNN
        (1-\sigma)\|c_k\|_1 < (\nabla f(x_k)^\top \dktrue + \max\{(\dktrue)^\top H_k \dktrue,0\}) \tau_{k-1}.
    \eequationNN
    
    By the definition of $\tau_k$, for any realization of $G_k$ such that\footnote{FEC: In this sentence, these should be $D_k$ and $G_k$, yes? MO: Honestly wasn't positive whether this should be in terms of a realization or a random variable. Made it more precise.}
    \bequationNN
        g_k^\top d_k + \max\{d_k^\top H_k d_k,0\} \geq \nabla f(x_k)^\top \dktrue + \max\{(\dktrue)^\top H_k \dktrue,0\}
    \eequationNN
    holds on an iteration such that $\tktritrue < \tau_{k-1}$, then
    \bequationNN
        (1-\sigma)\|c_k\|_1 < (g_k^\top d_k + \max\{d_k^\top H_k d_k,0\}) \tau_{k-1}
    \eequationNN
    occurs as well so that $\tau_k < \tau_{k-1}$. Noting that $\tktritrue < \tau_{k-1}$ is conditionally independent of $G_k$ given $\mathcal{F}_k$, it follows that
    \begin{align*}
        &\Prob[\Tcal_k < \tau_{k-1} |  \mathcal{F}_k, \tktritrue < \tau_{k-1}] \\
        &\geq \Prob[G_k^\top D_k + \max\{D_k^\top H_k D_k,0\} \geq \nabla f(x_k)^\top \dktrue + \max\{(\dktrue)^\top H_k \dktrue,0\} | \mathcal{F}_k, \tktritrue < \tau_{k-1}] \\
        &= \Prob[G_k^\top D_k + \max\{D_k^\top H_k D_k,0\} \geq \nabla f(x_k)^\top \dktrue + \max\{(\dktrue)^\top H_k \dktrue,0\} | \mathcal{F}_k] \\
        &\geq p_\tau.
    \end{align*}
    \qed
\eproof

Due to the above lemma, we can analyze the cardinality of $\Kcal_{\tau}$ by counting the number of $\tau$ decreases. In particular, by Lemma 2.16 of \cite{ABerahas_FECurtis_DPRobinson_BZhou_2021}, for any realization of the algorithm, there exists $\tau_{\min}^{\text{true}} > 0$\footnote{FEC: I guess we should add here that this is uniform over any run of the algorithm.} such that $\tktritrue \geq \min\{\tau_{\min}^{\text{true}},\tau_{k-1}\}$ at each iteration.\footnote{dpr:not sure why the $\tau_{k-1}$ is needed.  I am missing something.} Thus, let
\bequationNN
    \strue := \left\lceil \frac{\log(\tau_{\min}^{\text{true}}/\tau_{-1})}{\log(1-\epsilon)} \right\rceil,
\eequationNN
so that after $\strue$ decreases of $\tau$, it follows that\footnote{FEC: I don't understand the equality here.  Should it be an inequality? MO: Should be an inequality, messed up the trial value and the ``true" tau in my head.} $\tktritrue \geq \tau_{k-1} \geq \tau_{k}$ at each iteration.

Now, we introduce some Bernoulli random variables to aid in the analysis. Let $s_{\max} \in \N{}_{>0} \cup \{\infty\}$ denote the maximum number of times that $\tau$ may decrease in {\it any} realization. Unlike in Appendix \ref{app:simple}, we have an infinite sequence of random variables. Due to this, we allow $s_{\max}$ to take the value of $\infty$ (in which case the $Z_k$ random variables defined below would be fully independent, as would the probability of $\tau_k$ decreasing at each iteration when conditioned on the filtration\footnote{FEC: Am I understanding this correctly?  You're saying that if $s_{\max} = \infty$, then the probability of $\tau_k < \tau_{k-1}$ conditioned on the filtration would be equal to the total probability of $\tau_k < \tau_{k-1}$?  To be honest, I'm not sure why that would be true, nor why it's needed. MO: I didn't want to have to assume the existence of $s_{\max}$. They become fully independent if there is no $s_{\max}$ when properly conditioned on the filtration (they are dependent when conditioned on the filtration if $s_{\max}$ is finite). I don't believe they would be equal to the total probability even in this case. One would have to integrate over all realizations to obtain the total probability (while this is w.r.t. a single realization).}).

For all $k \in \N{}$, let $Z_k$ be a Bernoulli random variable such that
\bequation \label{eq:zkdefapp2}
    \begin{split}
        &\Prob\left[Z_k=1\Bigg| \sum_{i=0}^{k-1} Z_i < s_{\max}\right] = p_k \\
        \textrm{and} \; &\Prob\left[Z_k=1\Bigg| \sum_{i=0}^{k-1} Z_i \geq s_{\max}\right] = 0.
    \end{split}
\eequation

A useful property of these variables is derived below.

\begin{lemma} \label{lem:zindextra}
    Let $j \in \N{} \cup \{\infty\}$, let $s_{\max} \in \N{}_{>0} \cup \{\infty\}$, and let $s \leq s_{\max}$. For all $k \in \{0,\dots,j\}$, let $Z_k$ be defined as in \eqref{eq:zkdefapp2} and let $\hat{Z}_k$ be independent Bernoulli random variables with $\Prob[\hat{Z}_k = 1] = p_k$. Then,
    \bequationNN
        \Prob\left[\sum_{k=0}^j Z_k < s\right] = \Prob\left[\sum_{k=0}^j \hat{Z}_k < s\right].
    \eequationNN
\end{lemma}

\bproof
    For all $k \in \{0,\dots,j\}$, let $\bar{Z}_k$ be a Bernoulli random variable which follows the distribution:
    \bequationNN 
        \bar{Z}_k := \bcases
        1 & \textrm{when } \hat{Z}_k = 1 \textrm{ and } \sum_{i=0}^{k-1} \bar{Z}_i < s_{\max} \\
        0 & \textrm{otherwise}.
        \ecases
    \eequationNN
    
  \bequationNN
    \P\left[\bar{Z}_k = 1 \Bigg| \sum_{i=0}^{k-1} \bar{Z}_i < s_{\max} \right] = 
    \P\left[ \hat{Z}_k = 1 \Bigg| \sum_{i=0}^{k-1} \bar{Z}_i < s_{\max} \right] = \P[\hat{Z}_k = 1] = p_k
  \eequationNN
   \footnote{FEC: What does ``the'' mean here?  Is there really a unique such random variable?  Or do you mean that you want to define $\bar{Z}_k$ according to a similar formula, but with $\hat{z}_k$ and $\bar{z}_i$ replaced by random variables on the right-hand side? MO: Second one, rewrote the definition to be in terms of random variables.} By the definition of $\hat{Z}_k$
    and the definition of $\bar{Z}_k$, it follows that
    \begin{align*}
        \Prob\left[\bar{Z}_k = 1 \Bigg| \sum_{i=0}^{k-1} \bar{Z}_i < s_{\max}\right] &= p_k, \\
        \textrm{and } \Prob\left[\bar{Z}_k = 1 \Bigg| \sum_{i=0}^{k-1} \bar{Z}_i \geq s_{\max}\right] &= 0.
    \end{align*}
    
    Therefore, by \eqref{eq:zkdefapp2},\footnote{FEC: Do you mean \eqref{eq:zkdefapp2}? MO: Yes} for all $k \in \{0,\dots,j\}$, $\bar{Z}_k$ is equivalent in distribution to $Z_k$. Now, by the definition of $\bar{Z}_k$, since $s \leq s_{\max}$, the event $\sum_{k=0}^j \hat{Z}_k < s$ occurs if and only if the event $\sum_{k=0}^j \bar{Z}_k < s$ occurs as well. Thus,
    \bequationNN
        \Prob\left[\sum_{k=0}^j \hat{Z}_k < s\right] = \Prob\left[ \sum_{k=0}^j \bar{Z}_k < s\right] = \Prob\left[ \sum_{k=0}^j Z_k < s\right],
    \eequationNN
    where the last equality holds because, for all $k \in \{0,\dots,j\}$, 
    $\bar{Z}_k$ and $Z_k$ are equivalent in distribution.
\eproof

Next, we use Chernoff's bound to get control over independent Bernoulli random variables with high probability.

\blemma \label{lem:chernoffextra}
    Let $\ell \in \N{}_{>0}$. For all $k \in \{0,\dots,\ell\}$, let $Y_k$ be an independent Bernoulli random variable.\footnote{FEC: Independent from what?  I guess you mean that we're defining a sequence of independent Bernoulli random variables. MO: Yeah, that's what I mean. Not sure of a great way to be more precise.} Then, for any $s \in \N{}_{>0}$,
    \bequationNN
        \mu_{\ell} := \sum_{j=0}^{\ell} \Prob[Y_j = 1] \geq s \ \ \implies \ \ \Prob\left[\sum_{j=0}^{\ell} Y_j \leq s\right] \leq \exp\left(\frac{-(\mu_{\ell}-s)^2}{2\mu_{\ell}}\right).
    \eequationNN
\elemma

\bproof
    By the multiplicative form of Chernoff's bound, for any $\delta \in [0,1]$,
    \bequationNN
        \Prob\left[\sum_{j=0}^\ell Y_j \leq (1-\delta)\mu_\ell \right] \leq \exp\left(\frac{-\delta^2\mu_\ell}{2}\right).
    \eequationNN
    Substituting $\delta = \frac{\mu_\ell-s}{\mu_\ell}$ (which is in [0,1] by assumption),
    \bequationNN
        \Prob\left[\sum_{j=0}^\ell Y_j \leq s \right] \leq \exp\left(\frac{-((\mu_\ell-s)/\mu_\ell)^2\mu_\ell}{2}\right) = \exp\left(\frac{-(\mu_\ell-s)^2}{2\mu_\ell}\right).
    \eequationNN
    
    \iffalse
    By assumption, for all $k \in \N{}_{>0}$, it follows that $\mu_k := \sum_{j=0}^k \Prob[Y_j = 1] \geq s - \epsilon_k$ for some $\epsilon_k \geq 0$ such that $\lim_{k\rightarrow \infty} \epsilon_k = 0$, so that $\lim_{k\rightarrow \infty} \mu_k = \mu$.\footnote{FEC: I guess we should add here that $\mu_k \to \mu$, since it's used later.} For any such $k$, by the multiplicative form of Chernoff's bound, for any $\delta \in [0,1]$,
    \bequationNN
        \Prob\left[\sum_{j=0}^k Y_j \leq (1-\delta)\mu_k \right] \leq \exp\left(\frac{-\delta^2\mu_k}{2}\right).
    \eequationNN
    Substituting $\delta = \frac{\mu_k-s+\epsilon_k}{\mu_k}$ (which is in [0,1] by assumption),
    \bequationNN
        \Prob\left[\sum_{j=0}^k Y_j \leq s-\epsilon_k \right] \leq \exp\left(\frac{-((\mu_k-s+\epsilon_k)/\mu_k)^2\mu_k}{2}\right) = \exp\left(\frac{-(\mu_k-s+\epsilon_k)^2}{2\mu_k}\right).
    \eequationNN
    Thus, taking the limit as $k \rightarrow \infty$ yields the result.
    \fi
\eproof

Prior to our next result, we introduce the following random index set.\footnote{FEC: This is a \emph{random} index set, yes?} \footnote{FEC: Is this an arbitrary $p_\tau$?  Or the one from Lemma~\ref{lem:tautrialextra}? MO: It's intended to be used as the same one from Lemma~\ref{lem:tautrialextra}. Everything except for the last result holds for arbitrary $p_{\tau}$, however.}
\bequation \label{eq:Kstruep}
    \Kcal_{\strue,p_\tau} := \left\{k \in \N{} : \Prob\left[Z_k = 1\Bigg|\sum_{j=0}^{k-1} Z_j < s_{\max}\right] \geq p_\tau, \sum_{j=0}^{k-1} Z_j < \strue\right\}.
\eequation
We note that when $Z_k$ is the indicator of the event that $\Tcal_k < \tau_{k-1}$, then this set is a superset of $\Kcal_{\tau}$ for a specific realization due to  the definition of $\strue$ and Lemma \ref{lem:tautrialextra}.\footnote{dpr:I do not follow this.  Does this hold for all realizations? MO: This would be for a specific realization. We will eventually integrate over all realizations.}

Now, we find a high probability bound on the cardinality of $\Kcal_{\strue,p_\tau}$.

\blemma \label{lem:cardkstruep}
    Let $s_{\max} \in \N{}_{>0} \cup \{\infty\}$ and, for all $k \in \N{}$, let $Z_k$ be defined as in \eqref{eq:zkdefapp2}. Let $s \geq \strue$ and let $\Kcal_{\strue,p_\tau}$ be defined in \eqref{eq:Kstruep}.
    Then,
    \bequationNN
        \Prob\left[\Big|\Kcal_{\strue,p_\tau}\Big| > \frac{s+1}{p_\tau}\right] \leq \exp\left(-\frac{(s-\strue)^2}{2s}\right).
    \eequationNN
\elemma

\bproof
    First presume that\footnote{FEC: Are we presuming two things here?  First, that the series is convergent, and second that the sum is less than $s$?  Or is the former something we need to assume separately? MO: Yeah, we are. I don't think it's particularly relevant whether it converges or diverges in this particular proof.}
    \bequationNN
        \mu := \sum_{k=0}^\infty \Prob\left[Z_k = 1 \Bigg| \sum_{j=0}^{k-1} Z_j < s_{\max}\right] < s.
    \eequationNN
    By the definition of $Z_k$, it follows that\footnote{FEC: Why does the first inequality hold? MO: Directly from the definition of $Z_k$, the largest probability it can take is when the sum is less than $s_{\max}$ (as it is 0 otherwise). The term to the left of the inequality is simply the sum of the $p_k$'s in the definition.}
    \bequationNN
        \mu := \sum_{k=0}^\infty \Prob\left[Z_k = 1 \Bigg| \sum_{j=0}^{k-1} Z_j < s_{\max}\right] \geq \sum_{k \in \Kcal_{\strue,p_\tau}} p_\tau = |\Kcal_{\strue,p_\tau}| p_\tau.
    \eequationNN
    Therefore,
    \bequationNN
        |\Kcal_{\strue,p_\tau}| \leq \frac{\mu}{p_\tau},
    \eequationNN
    so that the result holds deterministically in this case. Thus, for the remainder of the proof, we assume that $\mu \geq s \geq \strue$.
    
    Now, let $\ell$ \footnote{FEC: This $\ell$ is a random variable, yes? MO: Not in this case, it's defined directly by the definition of $Z_k$, which is deterministic. In the next lemma we will integrate over all realizations in which case (if it was written down there), it would be a random variable.} be the minimum iteration such that
    \footnote{dpr:not sure I get this either.  Inside summation is also not always well defined.}
    \bequationNN
        \sum_{k=0}^\ell \Prob\left[Z_k = 1 \Bigg| \sum_{j=0}^{k-1} Z_j < s_{\max}\right] \geq s.
    \eequationNN
    By Lemmas \ref{lem:zindextra} and \ref{lem:chernoffextra}, we have\footnote{dpr:first inequality looks like an equality to me!}
    \bequationNN
        \Prob\left[\sum_{k=0}^{\ell} Z_k < \strue \right] = \Prob\left[\sum_{k=0}^{\ell} \hat{Z}_k < \strue \right] \leq \Prob\left[\sum_{k=0}^{\ell} \hat{Z}_k \leq \strue \right] \leq \exp\left(\frac{-(\mu_{\ell}-\strue)^2}{2\mu_{\ell}}\right).
    \eequationNN
    We note that $\exp(-(\mu_{\ell}-\strue)^2/2\mu_{\ell})$ is a decreasing function of $\mu_{\ell}$ for all $\mu_{\ell} \geq \strue$.
    Thus, by the definition of $\Kcal_{\strue,p_\tau}$,
    \bequationNN
      \baligned
        \Prob\left[\sum_{k=\ell+1}^{\infty} \Ical[k \in \Kcal_{\strue,p_\tau}] > 0\right] 
        &\leq \Prob\left[\sum_{k=\ell+1}^{\infty} \Ical\left[\sum_{j=0}^{k-1} Z_j < \strue\right] > 0\right] \\
        &\leq \Prob\left[\sum_{k=\ell+1}^{\infty} \Ical\left[\sum_{j=0}^{\ell} Z_j < \strue\right] > 0\right] \\
        &=    \Prob\left[\sum_{j=0}^{\ell} Z_j < \strue\right] \\
        &\leq \exp\left(\frac{-(\mu_{\ell}-\strue)^2}{2\mu_{\ell}}\right) \leq \exp\left(\frac{-(s-\strue)^2}{2s}\right),
      \ealigned
    \eequationNN
    where $\Ical[E]$ is the indicator function for the event $E$.
    In addition, by the definitions of $\Kcal_{\strue,p_\tau}$ and $\ell$, \footnote{FEC: Same question as before for the middle inequality.  Why does it hold? MO: See comment above, it's from the definition of $Z_k$.}
    \bequationNN
        s+1 \geq \sum_{k=0}^\ell \Prob\left[Z_k = 1 \Bigg| \sum_{j=0}^{k-1} Z_j < s_{\max}\right] \geq \sum_{k=0}^\ell \Ical[k \in \Kcal_{\strue,p_\tau}] p_\tau.
    \eequationNN
    Putting these together, we have
     \bequationNN
        \Prob\left[|\Kcal_{\strue,p_\tau}| > \frac{s+1}{p_\tau}\right] \leq \exp\left(\frac{-(s-\strue)^2}{2s}\right).
    \eequationNN
\eproof

Finally, we use the previous lemma and Lemma \ref{lem:tautrialextra} to derive a high-probability bound on $\Kcal_{\tau}$. Taking the limit of this result as $s \rightarrow \infty$ (after some slight rearranging) proves that $\Prob[|\Kcal_{\tau}| < \infty] = 1$.

\blemma
    Let the assumptions of \cite{ABerahas_FECurtis_DPRobinson_BZhou_2021} hold and let
    \bequationNN
        \Prob_k[G_k^\top D_k + \max\{D_k^\top H_k D_k,0\} \geq \nabla f(x_k)^\top \dktrue + \max\{(\dktrue)^\top H_k \dktrue,0\}] \geq p_\tau.
    \eequationNN
    Let $s \geq \strue$. Then,
    \bequationNN
        \Prob\left[\Big|\Kcal_{\tau}\Big| > \frac{s+1}{p_\tau}\right] \leq \exp\left(\frac{-(s-\strue)^2}{2s}\right). 
    \eequationNN
\elemma

\bproof
        Let $Z_k$ be the indicator of the event that $\Tcal_k < \tau_{k-1}$, let $P_k = \Prob[Z_k = 1 | \mathcal{F}_k, S_{k-1} < s_{\max}]$, and $P = \{P_0,P_1,\dots\}$. Additionally, let
        \bequationNN
            \Kcal_{\strue,p_\tau} := \left\{k \in \N{} : \Prob\left[\Tcal_k < \tau_{k-1}\Bigg|\sum_{j=0}^{k-1} \Ical[\Tcal_j < \tau_{j-1}]\right] \geq p_\tau, \sum_{j=0}^{k-1} \Ical[\Tcal_j < \tau_{j-1}] < \strue\right\}.
        \eequationNN
        Then, by Lemma \ref{lem:cardkstruep} and the definition of $s_{\max}$, it follows that
    \bequationNN
        \Prob\Bigg[\Big|\Kcal_{\strue,p_\tau}\Big| > \frac{s+1}{p_\tau} \Bigg| \left\{P_0, P_1, \dots \right\}
        = \left\{p_0,p_1,\dots\right\}\Bigg] \leq \exp\left(\frac{-(s-\strue)^2}{2s}\right),
    \eequationNN
    holds for any $p = \{p_0,p_1,\dots\}$ which is measurable with respect to the filtration $\mathcal{F}_{k_{\max}}$. Therefore by the law of total probability, for any $p = \{p_0,p_1,\dots\}$ which is measurable with respect to the filtration $\mathcal{F}_{k_{\max}}$,
    \begin{align*}
        &\Prob\left[\Big|\Kcal_{\strue,p_\tau}\Big| > \frac{s+1}{p_\tau}\right] \\
        &=\int_{p} \Prob\Bigg[\Big|\Kcal_{\strue,p_\tau}\Big| > \frac{s+1}{p_\tau} \Bigg| \left\{P_0, P_1, \dotsc, \right\} 
        = \left\{p_0, p_1, \dotsc\right\}\Bigg] f_P(p) dp \\
        &\leq \exp\left(\frac{-(s-\strue)^2}{2s}\right) \int_{p} f_{P}(p) dp = \exp\left(\frac{-(s-\strue)^2}{2s}\right),
    \end{align*}
    where $f_P$ is the probability density function of the random variable $P$.\footnote{FEC: What is $P$? MO: Defined it above, it's the sequence of $P_k$ random variables we are integrating over.}
    
    To see the final result, recall that by the definitions of $\tktritrue$ and $\strue$, if $\tau$ has been decreased at least $\strue$ times at iteration $j$, $\tktritrue \geq \tau_{k-1}$ holds at all iterations $k \geq j$. In addition, by Lemma \ref{lem:tautrialextra}, it follows that
    \bequationNN
        \Prob\left[\Tcal_k < \tau_{k-1} | \Fcal_k, \tktritrue < \tau_{k-1}\right] \geq p_{\tau},
    \eequationNN
    so that
    \bequationNN
        \Kcal_{\tau} \subseteq \Kcal_{\strue,p_{\tau}}.
    \eequationNN
\eproof

The rest of the proof follows trivially from here by taking limits as $s \rightarrow \infty$ and noting that if $|\Kcal_{\tau}| = \infty$ with probability $0$, then $E_{\tau \gg 0}$ occurs with probabilty $0$ as well.

\section{dpr copied some things here}

\smallskip
\hrule
\smallskip
Begin: DPR version \\
Next, we define the tree that we use to prove the desired bound on the probability of $\Ebad$. We define a node in the tree at a depth of $k$ in terms of two vectors, $p_{[k]} := [p_0,\dots,p_k]$ and $w_{[k]} :=  [w_0,\dots,w_k]$.  In this manner, the root node has a depth of $0$ and is defined by $p_0$ and $w_{-1}=0$.\footnote{dpr:not sure why we start out at depth $0$ given this notation.  Can't we just start at first level for $k=2$?}  We say that the event $[G_0, \dots, G_{k-1}] \in N(p_{[k]},w_{[k-1]})$ occurs if\footnote{dpr: I think I understand what is going on, but I am not sure if this notation is the best choice. I need time to go through the rest and digest, I think.}
\begin{align*}
    &\Prob[\Tcal_k < \Tcal_{k-1} | E, G_0,\dots,G_{k-1}] = p_k, \\
    &S_{k-1} = \sum_{i=0}^{k-1} \Ical[\Tcal_i < \Tcal_{i-1}] = w_{k-1}, \\
    \text{and the event}\ \ &G_0,\dots,G_{k-2} \in N(p_{[k-1]},w_{[k-2]}) \ \ \text{occurs as well.}
\end{align*}
Essentially, the vector $p_{[k]}$ encodes the history of the probabilities of merit parameter decreasing at every iteration up to iteration $k$ while $w_{[k-1]}$ records the total number of merit parameter decreases at each iteration prior to iteration $k$.  Note that $p_{[k]}$ has one more element than $w_{[k-1]}$ since the probability of decreasing the merit parameter at iteration $k$ is known given the stochastic gradients up to iteration $k-1$, but the number of decreases up to the end of iteration $k$ is not known until $G_k$ is observed.  We also note that $S_{k-1}$ in this definition is defined as a part of our stochastic process in Section~\ref{subsec:assumptions}.

\smallskip
\hrule 
\smallskip
Begin: MO version \\
Next, we start to define the tree that we use to prove the desired bound on the probability of $\Ebad$. We define a node in the tree at a depth of $k$ in terms of two vectors, $p_{[k]} := [p_0,\dots,p_k]$ and $w_{[k-1]} :=  [w_0,\dots,w_{k-1}]$.  In this manner, the root node has a depth of $0$ and is defined by $p_0$ and $w_{-1}=0$.\footnote{dpr:not sure why we start out at depth $0$ given this notation.  Can't we just start at first level for $k=2$?}  We say $[G_0, \dots, G_{k-1}] \in N(p_{[k]},w_{[k-1]})$ if\footnote{dpr: I think I understand what is going on, but I am not sure if this notation is the best choice. I need time to go through the rest and digest, I think.}
\begin{align*}
    &\Prob[\Tcal_k < \Tcal_{k-1} | E, G_0,\dots,G_{k-1}] = p_k, \\
    &S_{k-1} = \sum_{i=0}^{k-1} \Ical[\Tcal_i < \Tcal_{i-1}] = w_{k-1}, \\
    \text{and}\ \ &G_0,\dots,G_{k-2} \in N(p_{[k-1]},w_{[k-2]}).
\end{align*}
Essentially, the vector $p_{[k]}$ encodes the history of the probabilities of merit parameter decreasing at every iteration up to iteration $k$ while $w_{[k-1]}$ records the total number of merit parameter decreases at each iteration prior to iteration $k$.  Note that $p_{[k]}$ has one more element than $w_{[k-1]}$ since the probability of decreasing the merit parameter at iteration $k$ is known given the stochastic gradients up to iteration $k-1$, but the number of decreases up to the end of iteration $k$ is not known until $G_k$ is observed.  We also note that $S_{k-1}$ in this definition is defined as a part of our stochastic process in Section~\ref{subsec:assumptions}.
%
%\hrule
%\smallskip

For any realization of our algorithm we can define $\wbar_i$ as the number of times the merit parameter was decreased to obtain $x_i$, and $\pbar_i$ as the probability that the merit parameter would be decreased during iteration $i$; we define the \emph{signature} of that realization as $(\pbar_0,\dots,\pbar_{\kmax+1},\wbar_0,\dots,\wbar_{\kmax+1})$. Therefore, the signature of any realization of our algorithm belongs to a unique element of the set of signatures
\begin{align*}
\Scal := 
\{(p_0,\dots,p_{\kmax+1}, 
   w_0,\dots,w_{\kmax+1}):  
   p_i \in\{1/N,2/N,\dots,1\} \ \text{and} \  
   w_i \in\{0,1,\dots,i\} \}
\end{align*}
which has cardinality $|\Scal| = N^{\kmax+1} (\kmax+1)(\kmax+2)/2$.
We now wish to define a tree based on the set of signatures whereby each node will contain a subset of all realizations of the algorithm. Let us now define this tree by describing the nodes and edges.
%\begin{itemize}
    %\item \textbf{Nodes.} 
Level $k$ (starting with $k=0$) of the tree has $N^k k(k+1)/2$ nodes denoted by
    $$
    \{\Ncal(p_0,\dots,p_k,w_0,\dots,w_k): p_i\in\{1/N,2/N,\dots,1\} \ \text{and} \  
   w_i \in\{0,1,\dots,i\}\}.
    $$
    We say that a given realization with signature $(\pbar_0,\dots,\pbar_{\kmax+1},\wbar_0,\dots,\wbar_{\kmax+1})$ is contained in node $\Ncal(p_0,\dots,p_k,w_0,\dots,w_k)$ if $\pbar_i = p_i$ and $\wbar_i = w_i$ for all $i\in\{0,\dots,k\}$. From this definition it follows that if a realization is in node $\Ncal(p_0,\dots,p_k,w_0,\dots,w_k)$ then that realization must also be in node $\Ncal(p_0,\dots,p_j,w_0,\dots,w_j)$ for all $j\leq \{0,\dots,k\}$.  Moreover, the set of \emph{all} realizations is a subset of a \emph{single} node at level zero. For example, let $N = 5$ and suppose that the probability that the merit parameter decreases during iteration $0$ is $2/5$.  Then, it follows that every realization is contained in $\Ncal(2/5,0)$, i.e., no realizations are contained in $\Ncal(1/5,0)$, $\Ncal(3/5,0)$, $\Ncal(4/5,0)$, and $\Ncal(1,0)$.

%    \item \textbf{Edges.} 
Edges are only drawn between nodes at adjacent levels. %In particular, n
Node $\Ncal(p_0,\dots,p_k,w_0,\dots,w_k)$ at level $k$ for $k\in\{0,1,\dots,\kmax\}$ is connected to node $\Ncal(\pbar_0,\dots,\pbar_{k+1},\wbar_0,\dots,\wbar_{k+1})$ at level $k+1$ if and only if $p_j = \pbar_j$ and $w_j = \wbar_j$ for all $j\in\{0,1,\dots,k\}$.
%\end{itemize}

\smallskip
\hrule
\fi
